# Supplementary material for: Some elementary components of the Hilbert scheme of points
Source: arXiv:1407.1440 ancillary file (2016-01-21)
Supplement: Supplementary file 1 [file case__1_5_3_4_0_.pdf]

# Case (1,5,3,4,0).

This file accompanies the paper *Some Elementary Components of the Hilbert Scheme of Points*, to appear in the *Rocky Mountain Journal of Mathematics*.

Author: Mark Huibregtse

Affiliation: Skidmore College .

Email address: mhuibreg@skidmore.edu .

This notebook contains the details of example 8.1 of the paper. The notebook can be executed cell-by-cell, or all at once by selecting **Evaluate Notebook** from the **Evaluation** menu.

Assign the number of variables  $n$ , the list of variables  $\{x_1, \dots, x_n\}$ , and the list of null substitutions  $\{x_1 \rightarrow 0, \dots, x_n \rightarrow 0\}$ .

```
n = 5;  
varList = Table[xi, {i, 1, n}];  
nullSubs = makeNullSubList[varList];
```

Make the lex-segment complement order ideal for Hilbert function (1,5,4,5,0), and the set of boundary monomials.

```
OO = makeOrderIdeal[{1, 5, 3, 4}, varList]  
{1, x1, x2, x3, x4, x5, x42, x4 x5, x52, x43, x42 x5, x4 x52, x53}  
  
μ = Length[OO]  
13  
  
bdry = bdryMonoms[OO, varList]  
{x12, x1 x2, x1 x3, x1 x4, x1 x5, x22, x2 x3, x2 x4, x2 x5, x32, x3 x4, x3 x5, x1 x42, x1 x4 x5,  
x1 x52, x2 x42, x2 x4 x5, x2 x52, x3 x42, x3 x4 x5, x3 x52, x1 x43, x1 x42 x5, x1 x4 x52, x1 x53, x2 x43,  
x2 x42 x5, x2 x4 x52, x2 x53, x3 x43, x3 x42 x5, x3 x4 x52, x3 x53, x44, x43 x5, x42 x52, x4 x53, x54}  
  
numBdry = Length[bdry]  
38
```

Form the sets of leading and trailing monomials LM and TM.

```
mins = minBdryMons[OO, bdry, varList]
{ $x_1^2$ ,  $x_1 x_2$ ,  $x_1 x_3$ ,  $x_1 x_4$ ,  $x_1 x_5$ ,  $x_2^2$ ,  $x_2 x_3$ ,
 $x_2 x_4$ ,  $x_2 x_5$ ,  $x_3^2$ ,  $x_3 x_4$ ,  $x_3 x_5$ ,  $x_4^2$ ,  $x_4^3 x_5$ ,  $x_4^2 x_5^2$ ,  $x_4 x_5^3$ ,  $x_5^4$ }

LM = Take[mins, 12]
{ $x_1^2$ ,  $x_1 x_2$ ,  $x_1 x_3$ ,  $x_1 x_4$ ,  $x_1 x_5$ ,  $x_2^2$ ,  $x_2 x_3$ ,  $x_2 x_4$ ,  $x_2 x_5$ ,  $x_3^2$ ,  $x_3 x_4$ ,  $x_3 x_5$ }

λ = Length[LM]
12

maxes = maxBasisMons[OO, bdry, varList]
{ $x_1$ ,  $x_2$ ,  $x_3$ ,  $x_4^3$ ,  $x_4^2 x_5$ ,  $x_4 x_5^2$ ,  $x_5^3$ }

TM = Take[maxes, -4]
{ $x_4^3$ ,  $x_4^2 x_5$ ,  $x_4 x_5^2$ ,  $x_5^3$ }

τ = Length[TM]
4
```

Randomly generate a short list of polynomials  $G$ , test for efficiency and  $\theta$ -efficiency, and make the associated border basis of the distinguished ideal associated to the short list.

To generate the example shown in section 8.1 of the paper, un-comment the assignment cell following the next, which generates a new example at random.

```
G = makeShortListOfIdealGenerators[LM, TM]
{ $x_1^2 + x_4^3 + x_4^2 x_5 - x_4 x_5^2 + x_5^3$ ,  $x_1 x_2 + x_4^3 - x_4^2 x_5 + x_4 x_5^2$ ,  $x_1 x_3 + x_4^3 - x_4^2 x_5 - x_4 x_5^2$ ,  $x_1 x_4 - x_4^3 - x_4^2 x_5$ ,
 $x_1 x_5 - x_4^2 x_5 + x_5^3$ ,  $x_2^2 + x_4^3 + x_4^2 x_5 + x_4 x_5^2 + x_5^3$ ,  $x_2 x_3 - x_4^2 x_5 - x_4 x_5^2$ ,  $x_2 x_4 - x_4^3 + x_4^2 x_5 + x_4 x_5^2 + x_5^3$ ,
 $-x_4^3 + x_2 x_5 - x_4 x_5^2$ ,  $x_3^2 - x_4^3$ ,  $x_3 x_4 + x_4^3 + x_4^2 x_5 - x_4 x_5^2$ ,  $-x_4^3 + x_3 x_5 - x_4^2 x_5 + x_4 x_5^2 - x_5^3$ }
```

The following cell contains the example shown in Section 8.1 of the paper. To use it, just un-comment the cell and shift-enter it, then continue executing the remaining cells in the notebook.

```
(*G={ $x_1^2 - x_4^3 - x_4^2 x_5 + x_4 x_5^2 + x_5^3$ ,  $x_1 x_2 - x_4^3 + x_4^2 x_5 + x_4 x_5^2 + x_5^3$ ,
 $x_1 x_3 - x_4^2 x_5 + x_5^3$ ,  $x_1 x_4 + x_4^3 + x_4^2 x_5 - x_5^3$ ,  $x_1 x_5 + x_4^2 x_5 - x_5^3$ ,
 $x_2^2 + x_4^3 + x_4^2 x_5 + x_4 x_5^2 - x_5^3$ ,  $x_2 x_3 - x_4^3 - x_4^2 x_5$ ,  $x_2 x_4 + x_4^3 - x_4^2 x_5$ ,  $x_2 x_5 - x_4^2 x_5$ ,
 $x_3^2 + x_4^3 + x_4^2 x_5 + x_4 x_5^2 - x_5^3$ ,  $x_3 x_4 + x_4^3 - x_4^2 x_5$ ,  $x_3 x_5 - x_4^2 x_5 - x_4 x_5^2$ } ;
*)

Length[G]
12
```

```
isEfficient[G, LM, bdry, varList]
```

```
True
```

```
isThetaEfficient[G, LM, TM, bdry, varList, verbose = True]
```

```
Condition 1 of Proposition 3.1 is True.
```

```
(numProds = 60) >= (numQ = 48)
```

```
The map  $\varphi$  is surjective.
```

```
True
```

```
borBasis = makeBorderBasisOfI[G, bdry, LM]
```

```
{x1^2 + x4^3 + x4^2 x5 - x4 x5^2 + x5^3, x1 x2 + x4^3 - x4^2 x5 + x4 x5^2, x1 x3 + x4^3 - x4^2 x5 - x4 x5^2, x1 x4 - x4^3 - x4^2 x5,
x1 x5 - x4^2 x5 + x5^3, x2^2 + x4^3 + x4^2 x5 + x4 x5^2 + x5^3, x2 x3 - x4^2 x5 - x4 x5^2, x2 x4 - x4^3 + x4^2 x5 + x4 x5^2 + x5^3,
-x4^3 + x2 x5 - x4 x5^2, x3^2 - x4^3, x3 x4 + x4^3 + x4^2 x5 - x4 x5^2, -x4^3 + x3 x5 - x4^2 x5 + x4 x5^2 - x5^3, x1 x4^2,
x1 x4 x5, x1 x5^2, x2 x4^2, x2 x4 x5, x2 x5^2, x3 x4^2, x3 x4 x5, x3 x5^2, x1 x4^3, x1 x4^2 x5, x1 x4 x5^2, x1 x5^3,
x2 x4^3, x2 x4^2 x5, x2 x4 x5^2, x2 x5^3, x3 x4^3, x3 x4^2 x5, x3 x4 x5^2, x3 x5^3, x4^4, x4^3 x5, x4^2 x5^2, x4 x5^3, x5^4}
```

Find the tangent space relations and the dimension of the tangent space at  $[I]$ :

```
{aLst, allTanSpaceRelns} = makeTanSpaceRelns[borBasis, OO, bdry, varList];
```

```
tanSpaceDim[Length[aLst], allTanSpaceRelns]
```

```
59
```

As shown in Section 8.1 of the paper, a tangent space dimension of 59 implies that the ideal  $I = (G) = (\text{borBasis})$  is generic: The point  $[I]$  is a smooth point on an elementary component of dimension 59.

## Example showing that a generic distinguished ideal need not be efficient.

The following example was generated on Saturday, 9/21/2013. It shows that one can find a generic ideal of shape (1,5,3,4,0) that is not efficient. The cell immediately following contains the example in text form, for safe-keeping.

```
(*G={x1^2-x4^3+x4^2 x5+x5^3, x1 x2+x4^3-x4^2 x5+x4 x5^2, x1 x3-x4^3-x4^2 x5+x4 x5^2, x1 x4+x4^3-x4^2 x5,
x1 x5-x4^2 x5+x4 x5^2-x5^3, x2^2+x4^3+x4^2 x5+x4 x5^2, x2 x3+x4^2 x5-x4 x5^2, x2 x4-x4^2 x5,
-x4^3+x2 x5-x4^2 x5-x4 x5^2, x3^2-x4^3, x3 x4+x4^3+x4^2 x5-x4 x5^2, x4^3+x3 x5+x4^2 x5}*)
```

```
G = {x1^2 - x4^3 + x4^2 x5 + x5^3, x1 x2 + x4^3 - x4^2 x5 + x4 x5^2, x1 x3 - x4^3 - x4^2 x5 + x4 x5^2, x1 x4 + x4^3 - x4^2 x5,
x1 x5 - x4^2 x5 + x4 x5^2 - x5^3, x2^2 + x4^3 + x4^2 x5 + x4 x5^2, x2 x3 + x4^2 x5 - x4 x5^2, x2 x4 - x4^2 x5,
-x4^3 + x2 x5 - x4^2 x5 - x4 x5^2, x3^2 - x4^3, x3 x4 + x4^3 + x4^2 x5 - x4 x5^2, x4^3 + x3 x5 + x4^2 x5};
```

```

isEfficient[G, LM, bdry, varList]

False

isThetaEfficient[G, LM, TM, bdry, varList, verbose = True]

Condition 1 of Proposition 3.1 is True.

(numProds = 60) >= (numQ = 48)

The map  $\vartheta$  is not surjective.

False

borBasis = makeBorderBasisOfI[G, bdry, LM]

 $\{x_1^2 - x_4^3 + x_4^2 x_5 + x_5^3, x_1 x_2 + x_4^3 - x_4^2 x_5 + x_4 x_5^2, x_1 x_3 - x_4^3 - x_4^2 x_5 + x_4 x_5^2, x_1 x_4 + x_4^3 - x_4^2 x_5,$ 
 $x_1 x_5 - x_4^2 x_5 + x_4 x_5^2 - x_5^3, x_2^2 + x_4^3 + x_4^2 x_5 + x_4 x_5^2, x_2 x_3 + x_4^2 x_5 - x_4 x_5^2, x_2 x_4 - x_4^2 x_5,$ 
 $-x_4^3 + x_2 x_5 - x_4^2 x_5 - x_4 x_5^2, x_2^3 - x_4 x_5^2, x_3 x_4 + x_4^3 + x_4^2 x_5 - x_4 x_5^2, x_4^3 + x_3 x_5 + x_4^2 x_5, x_1 x_4^2,$ 
 $x_1 x_4 x_5, x_1 x_5^2, x_2 x_4^2, x_2 x_4 x_5, x_2 x_5^2, x_3 x_4^2, x_3 x_4 x_5, x_3 x_5^2, x_1 x_4^3, x_1 x_4^2 x_5, x_1 x_4 x_5^2, x_1 x_5^3,$ 
 $x_2 x_4^3, x_2 x_4^2 x_5, x_2 x_4 x_5^2, x_2 x_5^3, x_3 x_4^3, x_3 x_4^2 x_5, x_3 x_4 x_5^2, x_3 x_5^3, x_4^4, x_4^3 x_5, x_4^2 x_5^2, x_4 x_5^3, x_5^4\}$ 

nbrSyz = makeLinearSyzygies[bdry, borBasis, varList];

DeleteDuplicates[Table[Simplify[nbrSyz[[i]].borBasis], {i, 1, Length[nbrSyz]}]]

{0}

```

Find the tangent space relations and the dimension of the tangent space at  $[I]$ :

```

{aLst, allTanSpaceRelns} = makeTanSpaceRelns[borBasis, OO, bdry, varList];

tanSpaceDim[Length[aLst], allTanSpaceRelns]

59

```

So we indeed have an example of a generic distinguished ideal that is not efficient.
