# Supplementary material for: Some elementary components of the Hilbert scheme of points
Source: arXiv:1407.1440 ancillary file (2016-01-21)
Supplement: Supplementary file 2 [file case__1_5_3_4_5_6_0_.pdf]

# Case (1,5,3,4,5,6,0).

This file accompanies the paper *Some Elementary Components of the Hilbert Scheme of Points*, to appear in the *Rocky Mountain Journal of Mathematics*.

Author: Mark Huibregtse

Affiliation: Skidmore College .

Email address: mhuibreg@skidmore.edu .

This notebook contains the details of the example presented in Section 8.2 of the paper.

Assign the number of variables  $n$ , the list of variables  $\{x_1, \dots, x_n\}$ , and the list of null substitutions  $\{x_1 \rightarrow 0, \dots, x_n \rightarrow 0\}$ .

```
n = 5;  
varList = Table[xi, {i, 1, n}];  
nullSubs = makeNullSubLst[varList];
```

Make the lex-segment complement order ideal for Hilbert function (1,5,3,4,5,6,0), and the set of boundary monomials.

```
OO = makeOrderIdeal[{1, 5, 3, 4, 5, 6}, varList]  
{1, x1, x2, x3, x4, x5, x42, x4 x5, x52, x43, x42 x5, x4 x52,  
x53, x44, x43 x5, x42 x52, x4 x53, x54, x45, x44 x5, x43 x52, x42 x53, x4 x54, x55}  
  
μ = Length[OO]  
24  
  
bdry = bdryMonoms[OO, varList]  
{x12, x1 x2, x1 x3, x1 x4, x1 x5, x22, x2 x3, x2 x4, x2 x5, x32, x3 x4, x3 x5, x1 x42, x1 x4 x5, x1 x52,  
x2 x42, x2 x4 x5, x2 x52, x3 x42, x3 x4 x5, x3 x52, x1 x43, x1 x42 x5, x1 x4 x52, x1 x53, x2 x43, x2 x42 x5,  
x2 x4 x52, x2 x53, x3 x43, x3 x42 x5, x3 x4 x52, x3 x53, x1 x44, x1 x43 x5, x1 x42 x52, x1 x4 x53, x1 x54,  
x2 x44, x2 x43 x5, x2 x42 x52, x2 x4 x53, x2 x54, x3 x44, x3 x43 x5, x3 x42 x52, x3 x4 x53, x3 x54, x1 x45,  
x1 x44 x5, x1 x43 x52, x1 x42 x53, x1 x4 x54, x1 x55, x2 x45, x2 x44 x5, x2 x43 x52, x2 x42 x53, x2 x4 x54, x2 x55,  
x3 x45, x3 x44 x5, x3 x43 x52, x3 x42 x53, x3 x4 x54, x3 x55, x46, x45 x5, x44 x52, x43 x53, x42 x54, x4 x55, x56}
```

```
numBdry = Length[bdry]
```

73

Form the sets of leading and trailing monomials LM and TM.

```
mins = minBdryMons[OO, bdry, varList]
{ x1^2, x1 x2, x1 x3, x1 x4, x1 x5, x2^2, x2 x3, x2 x4,
  x2 x5, x3^2, x3 x4, x3 x5, x4^2, x4 x5, x5^2, x4^3, x4^2 x5, x4 x5^2, x5^3 }

LM = Take[mins, 12]
{ x1^2, x1 x2, x1 x3, x1 x4, x1 x5, x2^2, x2 x3, x2 x4, x2 x5, x3^2, x3 x4, x3 x5 }

λ = Length[LM]
12

maxes = maxBasisMons[OO, bdry, varList]
{ x1, x2, x3, x4^5, x4^4 x5, x4^3 x5^2, x4^2 x5^3, x4 x5^4, x5^5 }

TM = Take[maxes, -6]
{ x4^5, x4^4 x5, x4^3 x5^2, x4^2 x5^3, x4 x5^4, x5^5 }

τ = Length[TM]
6
```

Randomly generate a short list of polynomials  $G$ , test for efficiency and  $\theta$ -efficiency, and make the associated border basis of the distinguished ideal associated to the short list.

To generate a new random example, execute the immediately-following cell. To re-run a previously-executed example that works (i.e., produces a generic ideal), un-comment the assignment cell that follows the next.

```
G = makeShortListOfIdealGenerators[LM, TM]
{ x1^2 + x4^3 x5^2 + x5^5, x1 x2 - x4^5 - x4^4 x5 - x4^2 x5^3 + x4 x5^4, x1 x3 + x4^5 + x4^3 x5^2 + x4 x5^4 - x5^5,
  x1 x4 + x4^4 x5 - x4 x5^4 - x5^5, -x4^5 + x1 x5 + x4^3 x5^2 + x4^2 x5^3 + x4 x5^4, x2^2 + x4^5 + x4^4 x5 + x4^3 x5^2 - x4^2 x5^3,
  x2 x3 - x4^3 x5^2 - x4 x5^4, x2 x4 - x4^5 - x4^4 x5 - x5^5, x4^5 + x2 x5 - x4^4 x5 - x4^3 x5^2 + x4 x5^4,
  x3^2 + x4^5 + x4^4 x5 - x4^2 x5^3 + x5^5, x3 x4 + x4^5 - x4^3 x5^2, x3 x5 - x4^3 x5^2 + x4 x5^4 }
```

The following cell contains an example that works. To use it, just un-comment the cell and shift-enter it, then continue executing the remaining cells in the notebook.

```
(* G = { x1^2 + x4^5 - x4^3 x5^2 + x4 x5^4 + x5^5, x1 x2 + x4^5 - x4^4 x5 - x4^2 x5^3 - x4 x5^4, x1 x3 + x4^5 + x4^3 x5^2,
  x1 x4 + x4^4 x5 + x4^3 x5^2 + x4^2 x5^3 + x4 x5^4, x4^5 + x1 x5 - x4^3 x5^2 + x4^2 x5^3 + x4 x5^4 - x5^5,
  x2 x3 - x4^5 - x4^4 x5 + x4^3 x5^2 + x4^2 x5^3 - x4 x5^4 + x5^5, x2 x4 + x4^5 - x4^4 x5 - x4^3 x5^2 + x4 x5^4, x2 x5 + x4^4 x5 + x4^3 x5^2 + x5^5,
  x3^2 + x4^5 - x4^3 x5^2 - x5^5, x3 x4 + x4^5 - x4^4 x5 + x4^3 x5^2 + x4^2 x5^3 + x4 x5^4, -x4^5 + x3 x5 - x4^3 x5^2 - x5^5 } *)
```

**Length[G]**

12

**isEfficient[G, LM, bdry, varList]**

True

**isThetaEfficient[G, LM, TM, bdry, varList, verbose = True]**

Condition 1 of Proposition 3.1 is True.

(numProds = 60) >= (numQ = 56)

The map  $\vartheta$  is surjective.

True

**borBasis = makeBorderBasisOfI[G, bdry, LM]**

$$\left\{ x_1^2 + x_4^3 x_5^2 + x_5^5, x_1 x_2 - x_4^5 - x_4^4 x_5 - x_4^2 x_5^3 + x_4 x_5^4, x_1 x_3 + x_4^5 + x_4^3 x_5^2 + x_4 x_5^4 - x_5^5, \right. \\ x_1 x_4 + x_4^4 x_5 - x_4 x_5^4 - x_5^5, -x_4^5 + x_1 x_5 + x_4^3 x_5^2 + x_4^2 x_5^3 + x_4 x_5^4, x_2^2 + x_4^5 + x_4^4 x_5 + x_4^3 x_5^2 - x_4^2 x_5^3, \\ x_2 x_3 - x_4^3 x_5^2 - x_4 x_5^4, x_2 x_4 - x_4^5 - x_4^4 x_5 - x_5^5, x_4^5 + x_2 x_5 - x_4^4 x_5 - x_4^2 x_5^3 + x_4 x_5^4, \\ x_3^2 + x_4^5 + x_4^4 x_5 - x_4^2 x_5^3 + x_5^5, x_3 x_4 + x_4^5 - x_4^3 x_5^2, x_3 x_5 - x_4^3 x_5^2 + x_4 x_5^4, x_1 x_4^2, x_1 x_4 x_5, x_1 x_5^2, \\ x_2 x_4^2, x_2 x_4 x_5, x_2 x_5^2, x_3 x_4^2, x_3 x_4 x_5, x_3 x_5^2, x_1 x_4^3, x_1 x_4^2 x_5, x_1 x_4 x_5^2, x_1 x_5^3, x_2 x_4^3, x_2 x_4^2 x_5, \\ x_2 x_4 x_5^2, x_2 x_5^3, x_3 x_4^3, x_3 x_4^2 x_5, x_3 x_4 x_5^2, x_3 x_5^3, x_1 x_4^4, x_1 x_4^3 x_5, x_1 x_4^2 x_5^2, x_1 x_4 x_5^3, x_1 x_5^4, \\ x_2 x_4^4, x_2 x_4^3 x_5, x_2 x_4^2 x_5^2, x_2 x_4 x_5^3, x_2 x_5^4, x_3 x_4^4, x_3 x_4^3 x_5, x_3 x_4^2 x_5^2, x_3 x_4 x_5^3, x_3 x_5^4, x_1 x_5^5, \\ x_1 x_4^4 x_5, x_1 x_4^3 x_5^2, x_1 x_4^2 x_5^3, x_1 x_4 x_5^4, x_1 x_5^5, x_2 x_4^5, x_2 x_4^4 x_5, x_2 x_4^3 x_5^2, x_2 x_4^2 x_5^3, x_2 x_4 x_5^4, x_2 x_5^5, \\ \left. x_3 x_4^5, x_3 x_4^4 x_5, x_3 x_4^3 x_5^2, x_3 x_4^2 x_5^3, x_3 x_4 x_5^4, x_3 x_5^5, x_4^6, x_4^5 x_5, x_4^4 x_5^2, x_4^3 x_5^3, x_4^2 x_5^4, x_4 x_5^5, x_5^6 \right\}$$

**Find the tangent space relations and the dimension of the tangent space at [I]:**

**{aLst, allTanSpaceRelns} = makeTanSpaceRelns[borBasis, OO, bdry, varList];**

**tanSpaceDim[Length[aLst], allTanSpaceRelns]**

104

As shown in Section 8.2 of the paper, a tangent space dimension of 104 implies that the ideal  $I = (G) = (\text{borBasis})$  is generic.
