# Supplementary material for: Some elementary components of the Hilbert scheme of points
Source: arXiv:1407.1440 ancillary file (2016-01-21)
Supplement: Supplementary file 3 [file case__1_6_10_10_5_0__first.pdf]

# Case (1,6,10,10,5,0) first.

This file accompanies the paper *Some Elementary Components of the Hilbert Scheme of Points*, to appear in the *Rocky Mountain Journal of Mathematics*.

Author: Mark Huibregtse

Affiliation: Skidmore College .

Email address: mhuibreg@skidmore.edu .

This is the first of three generic examples with Hilbert function (1, 6, 10, 10, 5, 0); it is presented in section 8.5.1 of the paper. In this case, all the leading monomials are greater than all the trailing monomials in lex order, so Corollary 7.5 implies that the set of vectors  $S \sim Z'$  is linearly independent. It turns out that the dimension of this set of vectors is 255, which is also the dimension of the tangent space at sufficiently general ideals  $I$  having the structure of this example. So we have a generic component of dimension 255.

Assign the number of variables  $n$ , the list of variables  $\{x_1, \dots, x_n\}$ , and the list of null substitutions  $\{x_1 \rightarrow 0, \dots, x_n \rightarrow 0\}$ .

```
n = 6;  
varList = Table[xi, {i, 1, n}];  
nullSubs = makeNullSubLst[varList];
```

Make the lex-segment complement order ideal for Hilbert function (1,6,10,10,5,0), and the set of boundary monomials.

```
OO = makeOrderIdeal[{1, 6, 10, 10, 5}, varList]  
{1, x1, x2, x3, x4, x5, x6, x32, x3 x4, x3 x5, x3 x6, x42, x4 x5, x4 x6, x52, x5 x6, x62, x43,  
x42 x5, x42 x6, x4 x52, x4 x5 x6, x4 x62, x53, x52 x6, x5 x62, x63, x54, x53 x6, x52 x62, x5 x63, x64}
```

```
μ = Length[OO]
```

```

bdry = bdryMonoms[OO, varList]

{
  x1^2, x1 x2, x1 x3, x1 x4, x1 x5, x1 x6, x2^2, x2 x3, x2 x4, x2 x5, x2 x6, x1 x3^2, x1 x3 x4,
  x1 x3 x5, x1 x3 x6, x1 x4^2, x1 x4 x5, x1 x4 x6, x1 x5^2, x1 x5 x6, x1 x6^2, x2 x3^2, x2 x3 x4,
  x2 x3 x5, x2 x3 x6, x2 x4^2, x2 x4 x5, x2 x4 x6, x2 x5^2, x2 x5 x6, x2 x6^2, x3^3, x3^2 x4, x3^2 x5,
  x3^2 x6, x3 x4^2, x3 x4 x5, x3 x4 x6, x3 x5^2, x3 x5 x6, x3 x6^2, x1 x4^2, x1 x4^2 x5, x1 x4^2 x6,
  x1 x4 x5^2, x1 x4 x5 x6, x1 x4 x6^2, x1 x5^3, x1 x5^2 x6, x1 x5 x6^2, x1 x6^3, x2 x4^2, x2 x4^2 x5, x2 x4^2 x6,
  x2 x4 x5^2, x2 x4 x5 x6, x2 x4 x6^2, x2 x5^3, x2 x5^2 x6, x2 x5 x6^2, x2 x6^3, x3 x4^2, x3 x4^2 x5, x3 x4^2 x6,
  x3 x4 x5^2, x3 x4 x5 x6, x3 x4 x6^2, x3 x5^3, x3 x5^2 x6, x3 x5 x6^2, x3 x6^3, x4^4, x4^3 x5, x4^3 x6, x4^2 x5^2,
  x4^2 x5 x6, x4^2 x6^2, x4 x5^3, x4 x5^2 x6, x4 x5 x6^2, x4 x6^3, x1 x5^4, x1 x5^3 x6, x1 x5^2 x6^2, x1 x5 x6^3,
  x1 x6^4, x2 x5^4, x2 x5^3 x6, x2 x5^2 x6^2, x2 x5 x6^3, x2 x6^4, x3 x5^4, x3 x5^3 x6, x3 x5^2 x6^2, x3 x5 x6^3,
  x3 x6^4, x4 x5^4, x4 x5^3 x6, x4 x5^2 x6^2, x4 x5 x6^3, x4 x6^4, x5^5, x5^4 x6, x5^3 x6^2, x5^2 x6^3, x5 x6^4, x6^5}

numBdry = Length[bdry]

107

```

## Form the sets of leading and trailing monomials LM and TM

```

mins = minBdryMons[OO, bdry, varList]

{
  x1^2, x1 x2, x1 x3, x1 x4, x1 x5, x1 x6, x2^2, x2 x3, x2 x4, x2 x5, x2 x6, x3^3, x3^2 x4,
  x3^2 x5, x3^2 x6, x3 x4^2, x3 x4 x5, x3 x4 x6, x3 x5^2, x3 x5 x6, x3 x6^2, x4^4, x4^3 x5, x4^3 x6, x4^2 x5^2,
  x4^2 x5 x6, x4^2 x6^2, x4 x5^3, x4 x5^2 x6, x4 x5 x6^2, x4 x6^3, x5^5, x5^4 x6, x5^3 x6^2, x5^2 x6^3, x5 x6^4, x6^5}

LM = Join[Take[mins, 21]]

{
  x1^2, x1 x2, x1 x3, x1 x4, x1 x5, x1 x6, x2^2, x2 x3, x2 x4, x2 x5, x2 x6,
  x3^3, x3^2 x4, x3^2 x5, x3^2 x6, x3 x4^2, x3 x4 x5, x3 x4 x6, x3 x5^2, x3 x5 x6, x3 x6^2}

λ = Length[LM]

21

maxes = maxBasisMons[OO, bdry, varList]

{
  x1, x2, x3^2, x3 x4, x3 x5, x3 x6, x4^3, x4^2 x5,
  x4^2 x6, x4 x5^2, x4 x5 x6, x4 x6^2, x5^4, x5^3 x6, x5^2 x6^2, x5 x6^3, x6^4}

TM = Join[Take[maxes, -11]]

{
  x4^3, x4^2 x5, x4^2 x6, x4 x5^2, x4 x5 x6, x4 x6^2, x5^4, x5^3 x6, x5^2 x6^2, x5 x6^3, x6^4}

τ = Length[TM]

11

```

Randomly generate a short list of polynomials  $G$ , test for efficiency and  $\theta$ -efficiency, and make the associated border basis of the distinguished ideal associated to the short list.

**G = makeShortListOfIdealGenerators[LM, TM]**

$$\left\{ \begin{aligned} & x_1^2 + x_4^2 x_5 + x_4 x_5^2 - x_5^4 + x_4^2 x_6 + x_5^3 x_6 + x_4 x_6^2 - x_5^2 x_6^2 - x_5 x_6^3 - x_6^4, \\ & x_1 x_2 + x_4^3 - x_4 x_5^2 - x_4^2 x_6 - x_4 x_5 x_6 - x_4 x_6^2 - x_5^2 x_6^2 - x_6^4, \\ & x_1 x_3 + x_4^3 - x_4^2 x_5 + x_5^3 x_6 - x_4 x_6^2 + x_5^2 x_6^2 + x_5 x_6^3 - x_6^4, \\ & x_1 x_4 - x_4^3 + x_4^2 x_5 + x_4 x_5^2 + x_5^4 - x_4^2 x_6 + x_4 x_6^2 + x_5^2 x_6^2 + x_5 x_6^3 - x_6^4, \\ & -x_4^3 + x_1 x_5 - x_4^2 x_5 - x_4 x_5^2 + x_5^4 - x_4 x_5 x_6 - x_5^3 x_6 + x_4 x_6^2 - x_5^2 x_6^2 + x_5 x_6^3 + x_6^4, \\ & x_4^3 - x_4^2 x_5 - x_4 x_5^2 + x_1 x_6 + x_4^2 x_6 + x_4 x_5 x_6 - x_5^3 x_6 - x_5^2 x_6^2 - x_5 x_6^3 - x_6^4, \\ & x_2^2 + x_4^3 + x_4 x_5^2 + x_5^4 + x_4 x_5 x_6 + x_4 x_6^2 + x_5^2 x_6^2 - x_5 x_6^3 + x_6^4, \\ & x_2 x_3 - x_4^3 - x_4^2 x_5 - x_4 x_5^2 + x_5^4 + x_4^2 x_6 + x_4 x_6^2 + x_5^2 x_6^2 - x_5 x_6^3, \\ & x_2 x_4 + x_4^3 + x_4^2 x_5 - x_5^4 + x_4^2 x_6 + x_5^3 x_6 - x_6^4, \quad -x_4^3 + x_2 x_5 + x_4^2 x_5 + x_4 x_5^2 - x_5^4 - x_4^2 x_6 - x_4 x_6^2 - x_5 x_6^3 + x_6^4, \\ & x_4 x_5^2 + x_2 x_6 + x_4^2 x_6 + x_4 x_5 x_6 + x_5^3 x_6 + x_4 x_6^2 - x_5 x_6^3, \quad x_3^3 + x_4^3 + x_4 x_5^2 - x_4 x_6^2 + x_5^2 x_6^2 + x_6^4, \\ & x_3^2 x_4 + x_4^2 x_5 + x_4 x_5^2 - x_4^2 x_6 - x_4 x_5 x_6 + x_5 x_6^3 + x_6^4, \quad x_3^2 x_5 - x_4^2 x_5 - x_4 x_5^2 + x_4^2 x_6 + x_4 x_5 x_6 + x_5^3 x_6 + x_5^2 x_6^2, \\ & -x_4^3 + x_4 x_5^2 + x_5^3 x_6 - x_4 x_5 x_6 - x_5^3 x_6 + x_4 x_6^2 + x_5^2 x_6^2 + x_5 x_6^3 + x_6^4, \\ & x_3 x_4^2 + x_4^3 + x_4^2 x_5 + x_4 x_5^2 + x_5^4 + x_4^2 x_6 + x_5^3 x_6 + x_4 x_6^2 - x_5^2 x_6^2 - x_5 x_6^3 - x_6^4, \\ & x_4^3 + x_3 x_4 x_5 - x_4 x_5^2 - x_5^4 + x_4^2 x_6 + x_4 x_5 x_6 - x_5^3 x_6 + x_4 x_6^2 - x_5^2 x_6^2 - x_5 x_6^3, \\ & -x_4^2 x_5 - x_5^4 + x_3 x_4 x_6 - x_5^3 x_6 + x_4 x_6^2 + x_5 x_6^3 - x_6^4, \\ & -x_4^3 + x_4^2 x_5 + x_3 x_5^2 + x_4 x_5^2 - x_5^4 - x_4^2 x_6 - x_4 x_5 x_6 - x_5^2 x_6^2 - x_5 x_6^3 + x_6^4, \\ & x_4^3 - x_4^2 x_5 - x_5^4 + x_3 x_5 x_6 - x_5^3 x_6 + x_4 x_6^2 + x_5^2 x_6^2 + x_5 x_6^3, \quad x_5^4 + x_4^2 x_6 + x_5^3 x_6 + x_3 x_6^2 - x_4 x_6^2 - x_5^2 x_6^2 + x_5 x_6^3 \} \end{aligned} \right\}$$

The following example, which works, was generated on 8/11/2013.

(\*

**G = {**  $x_1^2 + x_4 x_5^2 - x_4^2 x_6 - x_4 x_5 x_6 - x_4 x_6^2 - x_5^2 x_6^2 - x_5 x_6^3 - x_6^4, x_1 x_2 - x_4^3 + x_4 x_5^2 - x_4^2 x_6 + x_4 x_5 x_6 + x_4 x_6^2 - x_5^2 x_6^2 - x_5 x_6^3 - x_6^4, x_1 x_3 - x_4^3 + x_4^2 x_5 + x_5^3 x_6 - x_4 x_6^2 + x_5^2 x_6^2 + x_5 x_6^3 - x_6^4, x_1 x_4 - x_4^3 + x_4^2 x_5 + x_4 x_5^2 + x_5^4 - x_4^2 x_6 + x_4 x_6^2 + x_5^2 x_6^2 + x_5 x_6^3 - x_6^4, -x_4^3 + x_1 x_5 - x_4^2 x_5 - x_4 x_5^2 + x_5^4 - x_4 x_5 x_6 - x_5^3 x_6 + x_4 x_6^2 - x_5^2 x_6^2 + x_5 x_6^3 + x_6^4, x_4^3 - x_4^2 x_5 - x_4 x_5^2 + x_1 x_6 + x_4^2 x_6 + x_4 x_5 x_6 - x_5^3 x_6 - x_5^2 x_6^2 - x_5 x_6^3 - x_6^4, x_2^2 + x_4^3 + x_4 x_5^2 + x_5^4 + x_4 x_5 x_6 + x_4 x_6^2 + x_5^2 x_6^2 - x_5 x_6^3 + x_6^4, x_2 x_3 - x_4^3 - x_4^2 x_5 - x_4 x_5^2 + x_5^4 + x_4^2 x_6 + x_4 x_6^2 + x_5^2 x_6^2 - x_5 x_6^3, x_2 x_4 + x_4^3 + x_4^2 x_5 - x_5^4 + x_4^2 x_6 + x_5^3 x_6 - x_6^4, -x_4^3 + x_2 x_5 + x_4^2 x_5 + x_4 x_5^2 - x_5^4 - x_4^2 x_6 - x_4 x_6^2 - x_5 x_6^3 + x_6^4, x_4 x_5^2 + x_2 x_6 + x_4^2 x_6 + x_4 x_5 x_6 + x_5^3 x_6 + x_4 x_6^2 - x_5 x_6^3, x_3^3 + x_4^3 + x_4 x_5^2 - x_4 x_6^2 + x_5^2 x_6^2 + x_6^4, x_3^2 x_4 + x_4^2 x_5 + x_4 x_5^2 - x_4^2 x_6 - x_4 x_5 x_6 + x_5 x_6^3 + x_6^4, x_3^2 x_5 - x_4^2 x_5 - x_4 x_5^2 + x_4^2 x_6 + x_4 x_5 x_6 + x_5^3 x_6 + x_5^2 x_6^2, -x_4^3 + x_4 x_5^2 + x_5^3 x_6 - x_4 x_5 x_6 - x_5^3 x_6 + x_4 x_6^2 + x_5^2 x_6^2 + x_5 x_6^3 + x_6^4, x_3 x_4^2 + x_4^3 + x_4^2 x_5 + x_4 x_5^2 + x_5^4 + x_4^2 x_6 + x_5^3 x_6 + x_4 x_6^2 - x_5^2 x_6^2 - x_5 x_6^3 - x_6^4, x_4^3 + x_3 x_4 x_5 - x_4 x_5^2 - x_5^4 + x_4^2 x_6 + x_4 x_5 x_6 - x_5^3 x_6 + x_4 x_6^2 - x_5^2 x_6^2 - x_5 x_6^3, -x_4^2 x_5 - x_5^4 + x_3 x_4 x_6 - x_5^3 x_6 + x_4 x_6^2 + x_5 x_6^3 - x_6^4, -x_4^3 + x_4^2 x_5 + x_3 x_5^2 + x_4 x_5^2 - x_5^4 - x_4^2 x_6 - x_4 x_5 x_6 - x_5^2 x_6^2 - x_5 x_6^3 + x_6^4, x_4^3 - x_4^2 x_5 - x_5^4 + x_3 x_5 x_6 - x_5^3 x_6 + x_4 x_6^2 + x_5^2 x_6^2 + x_5 x_6^3, x_5^4 + x_4^2 x_6 + x_5^3 x_6 + x_3 x_6^2 - x_4 x_6^2 - x_5^2 x_6^2 + x_5 x_6^3$  **};** \*)

**Length[G]**

21

**isEfficient[G, LM, bdry, varList]**

True

**isThetaEfficient[G, LM, TM, bdry, varList, verbose = True]**

Condition 1 of Proposition 3.1 is True.

`(numProds = 126) >= (numQ = 124)`

The map  $\vartheta$  is not surjective.

False

`borBasis = makeBorderBasisOfI[G, bdry, LM];`

## Find the tangent space relations and the dimension of the tangent space at $[I]$

`{aLst, allTanSpaceRelns} = makeTanSpaceRelns[borBasis, OO, bdry, varList];`

`tanSpaceDim[Length[aLst], allTanSpaceRelns]`

255

As noted in section 8.5.1 of the paper, this dimension is the minimum possible, and the efficient ideal  $I = (G)$  is generic.
