# Supplementary material for: Some elementary components of the Hilbert scheme of points
Source: arXiv:1407.1440 ancillary file (2016-01-21)
Supplement: Supplementary file 4 [file case__1_6_10_10_5_0__second.pdf]

# Case (1,6,10,10,5,0) second.

This file accompanies the paper *Some Elementary Components of the Hilbert Scheme of Points*, to appear in the *Rocky Mountain Journal of Mathematics*.

Author: Mark Huibregtse

Affiliation: Skidmore College .

Email address: mhuibreg@skidmore.edu .

This is the second of three generic examples with Hilbert function (1, 6, 10, 10, 5, 0); it is presented in section 8.5.2 of the paper. In this case, some of the trailing monomials are lex-larger than some of the leading monomials, so Corollary 7.5 does not apply. On the other hand, we show by direct computation that the set of tangent vectors  $S \sim Z$  is linearly independent for sufficiently general distinguished ideals  $I$ . It turns out that the dimension of this set of vectors is 222, which accordingly (Corollary 7.7) is a lower bound on the dimension of an irreducible locus containing the point  $[I]$ . Since the dimension of the tangent space at  $[I]$  is also 222, it follows from Proposition 5.5 that  $I$  is generic.

Assign the number of variables  $n$ , the list of variables  $\{x_1, \dots, x_n\}$ , and the list of null substitutions  $\{x_1 \rightarrow 0, \dots, x_n \rightarrow 0\}$ .

```
n = 6;  
varList = Table[xi, {i, 1, n}];  
nullSubs = makeNullSubLst[varList];
```

Make the lex-segment complement order ideal for Hilbert function (1,6,10,10,5,0), and the set of boundary monomials.

```
OO = makeOrderIdeal[{1, 6, 10, 10, 5}, varList]  
{1, x1, x2, x3, x4, x5, x6, x32, x3 x4, x3 x5, x3 x6, x42, x4 x5, x4 x6, x52, x5 x6, x62, x43,  
x42 x5, x42 x6, x4 x52, x4 x5 x6, x4 x62, x53, x52 x6, x5 x62, x63, x54, x53 x6, x52 x62, x5 x63, x64}  
  
μ = Length[OO]  
32
```

```
bdry = bdryMonoms[OO, varList]
```

```
{x1^2, x1 x2, x1 x3, x1 x4, x1 x5, x1 x6, x2^2, x2 x3, x2 x4, x2 x5, x2 x6, x1 x3^2, x1 x3 x4,
  x1 x3 x5, x1 x3 x6, x1 x4^2, x1 x4 x5, x1 x4 x6, x1 x5^2, x1 x5 x6, x1 x6^2, x2 x3^2, x2 x3 x4,
  x2 x3 x5, x2 x3 x6, x2 x4^2, x2 x4 x5, x2 x4 x6, x2 x5^2, x2 x5 x6, x2 x6^2, x3^3, x3^2 x4, x3^2 x5,
  x3^2 x6, x3 x4^2, x3 x4 x5, x3 x4 x6, x3 x5^2, x3 x5 x6, x3 x6^2, x1 x4^3, x1 x4^2 x5, x1 x4^2 x6,
  x1 x4 x5^2, x1 x4 x5 x6, x1 x4 x6^2, x1 x5^3, x1 x5^2 x6, x1 x5 x6^2, x1 x6^3, x2 x4^3, x2 x4^2 x5, x2 x4^2 x6,
  x2 x4 x5^2, x2 x4 x5 x6, x2 x4 x6^2, x2 x5^3, x2 x5^2 x6, x2 x5 x6^2, x2 x6^3, x3 x4^3, x3 x4^2 x5, x3 x4^2 x6,
  x3 x4 x5^2, x3 x4 x5 x6, x3 x4 x6^2, x3 x5^3, x3 x5^2 x6, x3 x5 x6^2, x3 x6^3, x4^4, x4^3 x5, x4^3 x6, x4^2 x5^2,
  x4^2 x5 x6, x4^2 x6^2, x4 x5^3, x4 x5^2 x6, x4 x5 x6^2, x4 x6^3, x1 x4^5, x1 x5^3 x6, x1 x5^2 x6^2, x1 x5 x6^3,
  x1 x6^4, x2 x5^4, x2 x5^3 x6, x2 x5^2 x6^2, x2 x5 x6^3, x2 x6^4, x3 x5^4, x3 x5^3 x6, x3 x5^2 x6^2, x3 x5 x6^3,
  x3 x6^4, x4 x5^4, x4 x5^3 x6, x4 x5^2 x6^2, x4 x5 x6^3, x4 x6^4, x5^5, x4^4 x6, x3^3 x6^2, x5^2 x6^3, x5 x6^4, x6^5}
```

```
numBdry = Length[bdry]
```

```
107
```

## Form the sets of leading and trailing monomials LM and TM

```
mins = minBdryMons[OO, bdry, varList]
```

```
{x1^2, x1 x2, x1 x3, x1 x4, x1 x5, x1 x6, x2^2, x2 x3, x2 x4, x2 x5, x2 x6, x3^3, x3^2 x4,
  x3^2 x5, x3^2 x6, x3 x4^2, x3 x4 x5, x3 x4 x6, x3 x5^2, x3 x5 x6, x3 x6^2, x4^4, x4^3 x5, x4^3 x6, x4^2 x5^2,
  x4^2 x5 x6, x4^2 x6^2, x4 x5^3, x4 x5^2 x6, x4 x5 x6^2, x4 x6^3, x5^5, x4^4 x6, x3^3 x6^2, x5^2 x6^3, x5 x6^4, x6^5}
```

```
mins[[31]]
```

```
x4 x6^3
```

```
Length[mins]
```

```
37
```

```
LM = Join[Take[mins, 11], Take[mins, {22, 31}]]
```

```
{x1^2, x1 x2, x1 x3, x1 x4, x1 x5, x1 x6, x2^2, x2 x3, x2 x4, x2 x5, x2 x6,
  x4^4, x4^3 x5, x4^3 x6, x4^2 x5^2, x4^2 x5 x6, x4^2 x6^2, x4 x5^3, x4 x5^2 x6, x4 x5 x6^2, x4 x6^3}
```

```
λ = Length[LM]
```

```
21
```

```
maxes = maxBasisMons[OO, bdry, varList]
```

```
{x1, x2, x3^2, x3 x4, x3 x5, x3 x6, x4^3, x4^2 x5,
  x4^2 x6, x4 x5^2, x4 x5 x6, x4 x6^2, x5^4, x5^3 x6, x5^2 x6^2, x5 x6^3, x6^4}
```

```
TM = Join[Take[maxes, {3, 6}], Take[maxes, -5]]
```

```
{x3^2, x3 x4, x3 x5, x3 x6, x4^4, x4^3 x6, x5^2 x6^2, x5 x6^3, x6^4}
```

```
τ = Length[TM]
```

```
9
```

Randomly generate a short list of polynomials  $G$ , test for efficiency and  $\theta$ -efficiency, and make the associated border basis of the distinguished ideal associated to the short list.

To generate a new example, execute the cell immediately following. To use an example that works that was generated on 7/29/2013, un-comment the assignment statement and execute it instead.

```
G = makeShortListOfIdealGenerators[LM, TM]
```

```
{x1^2 - x3^2 + x3 x5 - x5^4 - x3 x6 - x5^3 x6 - x5^2 x6^2 - x5 x6^3,
 x1 x2 - x3^2 + x5^4 + x3 x6 + x5^3 x6 + x5^2 x6^2 + x5 x6^3 + x6^4, x1 x3 - x3 x4 - x3 x6 - x5 x6^2 + x6^4,
 x1 x4 - x3 x4 + x3 x5 - x3 x6 - x5^2 x6^2 - x5 x6^3 + x6^4, -x3^2 + x1 x5 + x3 x5 - x5^4 + x3 x6 - x5^3 x6 - x5^2 x6^2 - x5 x6^3,
 x3^2 + x5^4 + x1 x6 - x3 x6 + x5^2 x6^2 + x5 x6^3, x2^2 + x3^2 - x5^4 + x3 x6 - x5^2 x6^2 + x5 x6^3,
 x2 x3 + x3^2 + x3 x4 - x3 x5 - x5^4 - x5^2 x6^2, -x3^2 + x2 x4 + x3 x4 + x3 x5 - x5^4 - x3 x6 + x5^2 x6^2 - x6^4,
 -x3^2 + x2 x5 + x3 x5 - x5^4 + x3 x6 + x5^2 x6^2, -x3^2 - x3 x5 - x5^4 + x2 x6 - x3 x6 + x6^4,
 x3^2 + x3 x4 + x4^4 - x5^4 + x5^2 x6^2 + x6^4, x3^2 + x4^2 x5 + x5^4 - x3 x6 - x5^3 x6 + x5^2 x6^2 - x5 x6^3,
 x3^2 + x3 x4 - x3 x5 - x5^4 - x3 x6 + x4^2 x6 - x3^2 x6 - x5^2 x6^2 - x5 x6^3 - x6^4,
 -x3^2 - x3 x5 + x4^2 x5^2 - x5^4 + x3 x6 - x5^3 x6 - x5 x6^3 - x6^4,
 -x3 x5 + x5^4 - x3 x6 + x4^2 x5 x6 + x5^2 x6^2 - x5 x6^3 + x6^4, x3^2 + x3 x4 + x5^4 - x3 x6 + x4^2 x6^2 - x5^2 x6^2 + x5 x6^3 - x6^4,
 x3 x5 + x4 x5^2 + x5^4 - x3 x6 + x6^4, -x3 x5 - x3 x6 + x4 x5^2 x6 - x5^2 x6^2 - x5 x6^3 - x6^4,
 -x3 x4 + x3 x5 + x5^4 + x4 x5 x6^2 - x5^2 x6^2 + x5 x6^3, x5^4 + x3 x6 - x5^2 x6^2 + x5^2 x6^2 + x4 x6^3 - x5 x6^3 + x6^4}
```

Example generated on 3/07/2014 that works.

```
(* G={x1^2-x3^2+x3 x4+x3 x5+x5^4+x3 x6+x5^2 x6^2-x5 x6^3+x6^4,
 x1 x2-x3^2+x5^4-x3 x6-x5^3 x6-x5^2 x6^2-x6^4,x1 x3+x3 x4-x3 x5-x5^4-x3 x6+x5^3 x6-x5^2 x6^2-x5 x6^3+x6^4,
 x1 x4-x3 x4-x3 x5-x5^4+x3 x6+x5^2 x6^2+x5 x6^3+x6^4,x3 x4+x1 x5-x3 x5+x5^4+x5^3 x6-x5^2 x6^2-x5 x6^3,
 -x3 x4-x3 x5+x5^4+x1 x6-x3 x6-x5^2 x6^2-x6^4,x2^2-x3^2-x3 x4-x3 x5+x5^4+x3 x6-x5 x6^3-x6^4,
 x2 x3+x3^2-x3 x4-x3 x5-x5^4-x3 x6+x5^3 x6-x5^2 x6^2-x5 x6^3-x6^4,
 x3^2+x2 x4+x3 x4+x3 x5-x5^4-x3 x6+x5^3 x6-x5^2 x6^2-x6^4,x2 x5-x3 x5+x5^4-x3 x6-x5^2 x6^2+x6^4,
 -x3^2+x3 x4-x3 x5+x2 x6-x3 x6-x5^3 x6-x5^2 x6^2+x5 x6^3+x6^4,x3^2+x3 x4+x4^4-x5^4+x5^3 x6+x5 x6^3+x6^4,
 x3^2-x3 x4-x3 x5+x4^2 x5-x3 x6-x5 x6^3+x6^4,x3 x4+x5^4+x3 x6+x4^2 x6-x6^4,x3 x4+x4^2 x5^2-x5^4+x5^3 x6+x6^4,
 x3^2+x3 x4-x3 x5-x5^4+x3 x6+x4^2 x5 x6-x5^2 x6^2+x5 x6^3-x6^4,-x3^2-x5^4-x5^3 x6+x4^2 x6^2-x5^2 x6^2,
 -x3^2-x3 x4+x4 x5^2+x5^4+x5^3 x6-x5^2 x6^2-x6^4,x3^2-x3 x5+x4 x5^2 x6+x5^3 x6+x5^2 x6^2+x5 x6^3+x6^4,
 x3^2+x3 x6+x5^3 x6+x4 x5 x6^2+x5^2 x6^2+x6^4,-x3^2-x3 x4-x3 x5+x5^4-x5^2 x6^2+x4 x6^3-x5 x6^3}; *)
```

```
Length[G]
```

```
21
```

```
isEfficient[G, LM, bdry, varList]
```

```
True
```

```
isThetaEfficient[G, LM, TM, bdry, varList, verbose = True]
```

```
Condition 1 of Proposition 3.1 is True.
```

```
(numProds = 126) >= (numQ = 112)
```

```
The map  $\vartheta$  is surjective.
```

```
True
```

```
borBasis = makeBorderBasisOfI[G, bdry, LM];
```

## Find the tangent space relations and the dimension of the tangent space at $[I]$

```
{aLst, allTanSpaceReIns} = makeTanSpaceReIns[borBasis, OO, bdry, varList];
```

```
tanSpaceDim[Length[aLst], allTanSpaceReIns]
```

```
222
```

As shown in Section 8.5.2 of the paper, the set of tangent vectors  $S \cup Z$  has cardinality 222. If we can show that these vectors are linearly independent at  $[I]$ , then we will know that the dimension of the locus  $F(U)$  is  $\geq 222$ ; whence,  $I$  is generic and  $[I]$  is smooth on an elementary component of dimension 222. In the next section of the notebook, we compute the tuples  $(a_{ij})$  corresponding to the tangent vectors in  $S \cup Z$  and show by direct computation that they are linearly independent. We need to do this computationally, since we don't have any general theorems stating when  $S \cup Z$  is linearly independent.

The tuples are produced by following the "recipe" given in equation (22) of section 6.2 of the paper.

---

## Create explicit vectors in our 6 translation directions

### $x_\alpha$ -translations, $1 \leq \alpha \leq 6$ :

The following function makes the tuples corresponding to the  $n$  tangent vectors given by translating in the  $x_1, \dots, x_n$ -directions.

```
makeTranslationVector[var_] := Flatten[
  Table[coeffOfTerm[ reducePoly[D[borBasis[[j]], var], bdry, borBasis, varList] ,
    OO[[i]] , varList], {j, 1, numBdry}, {i, 1,  $\mu$ }, 1];
```

```
x1trans = makeTranslationVector[x1];
```

```
Length[x1trans]
```

```
3424
```

```
numBdry *  $\mu$ 
```

```
3424
```

```

x2trans = makeTranslationVector[x2];
x3trans = makeTranslationVector[x3];
x4trans = makeTranslationVector[x4];
x5trans = makeTranslationVector[x5];
x6trans = makeTranslationVector[x6];

```

Executing the following cell for **x1trans** through **x6trans** will demonstrate that these tuples are indeed tangent vectors at  $[I]$ , since they satisfy all of the tangent space relations. (The result should be  $\{0\}$ .)

```

DeleteDuplicates[
  Table[allTanSpaceReIns[[i]].x2trans, {i, 1, Length[allTanSpaceReIns]}]]
{0}

MatrixRank[transVectors = {x1trans, x2trans, x3trans, x4trans, x5trans, x6trans}]

```

6

## Now we need to construct the remaining tangent vectors in $Z$ .

These tangent vectors correspond to the isomorphisms defined by the replacements  $(x_\alpha \rightarrow x_\alpha + m_{\{\alpha, \delta\}})$ . These are obtained by taking the partial of each member of the border basis with respect to  $x_\alpha$  and then multiplying by  $m_{\{\alpha, \delta\}}$  before taking the coefficients modulo  $I$ .

To reduce modulo  $I$ , we will use the function **reducePoly**. Because of the way the function **reducePoly** is coded, we will have to multiply by the variables appearing in  $m_{\{\alpha, \delta\}}$  one-by-one, reducing as we go. So the monomials will be entered as lists of variables which multiply to yield the monomial.

The inputs to the following function are: poly = one of the elements of the border basis; var =  $x_i$  -- the variable in the substitution  $x_i \rightarrow x_i + m$ ; and mon, the monomial  $m$  in the form of a list of the variables that constitute  $m$ : for example,  $m = x_2 x_3$  is entered as the list  $\{x_2, x_3\}$ . The output is the partial derivative of poly with respect to the given variable var multiplied by the given monomial mon, and then reduced modulo  $I$  (which results in a linear combination of the basis monomials).

```

parDerivTimesMonom[poly_, var_, mon_] := Module[{curVar, monDeg, result, i},
  (
    monDeg = Length[mon];
    result = reducePoly[D[poly, var], bdry, borBasis, varList];
    For[i = 1, i ≤ monDeg, i++,
      (
        curVar = mon[[i]];
        result = reducePoly[result * curVar, bdry, borBasis, varList];
      )];
    result
  )];

makeSubstitutionVector[var_, mon_] :=
  Flatten[Table[coeffOfTerm[ parDerivTimesMonom[borBasis[[j]], var, mon] ,
    OO[[i]], varList ], {j, 1, numBdry}, {i, 1,  $\mu$ }], 1];

sub14 = makeSubstitutionVector[x1, {x4}];
sub15 = makeSubstitutionVector[x1, {x5}];
sub16 = makeSubstitutionVector[x1, {x6}];
sub144 = makeSubstitutionVector[x1, {x4, x4}];
sub145 = makeSubstitutionVector[x1, {x4, x5}];
sub146 = makeSubstitutionVector[x1, {x4, x6}];
sub155 = makeSubstitutionVector[x1, {x5, x5}];
sub156 = makeSubstitutionVector[x1, {x5, x6}];
sub166 = makeSubstitutionVector[x1, {x6, x6}];
sub24 = makeSubstitutionVector[x2, {x4}];
sub25 = makeSubstitutionVector[x2, {x5}];
sub26 = makeSubstitutionVector[x2, {x6}];
sub244 = makeSubstitutionVector[x2, {x4, x4}];
sub245 = makeSubstitutionVector[x2, {x4, x5}];
sub246 = makeSubstitutionVector[x2, {x4, x6}];
sub255 = makeSubstitutionVector[x2, {x5, x5}];
sub256 = makeSubstitutionVector[x2, {x5, x6}];
sub266 = makeSubstitutionVector[x2, {x6, x6}];
sub34 = makeSubstitutionVector[x3, {x4}];

```

```

sub35 = makeSubstitutionVector[x3, {x5}];
sub36 = makeSubstitutionVector[x3, {x6}];
sub344 = makeSubstitutionVector[x3, {x4, x4}];
sub345 = makeSubstitutionVector[x3, {x4, x5}];
sub346 = makeSubstitutionVector[x3, {x4, x6}];
sub355 = makeSubstitutionVector[x3, {x5, x5}];
sub356 = makeSubstitutionVector[x3, {x5, x6}];
sub366 = makeSubstitutionVector[x3, {x6, x6}];

MatrixRank[
  zTuples = Join[transVectors, {sub14, sub15, sub16, sub144, sub145, sub146, sub155,
    sub156, sub166, sub24, sub25, sub26, sub244, sub245, sub246, sub255, sub256,
    sub266, sub34, sub35, sub36, sub344, sub345, sub346, sub355, sub356, sub366}]]

```

33

As above, the following line can be executed for any of the tuples in the preceding list to verify that it (the chosen tuple) is indeed a tangent vector at [/].

```

DeleteDuplicates[
  Table[allTanSpaceReIns[[i]].sub246, {i, 1, Length[allTanSpaceReIns]}]]
{0}

```

Now we create the tuples of the tangent vectors that lie in  $S$ , the tangent vectors that correspond to tweaking the coefficients of the short list of generators  $G$ .

This is easy to do, at least conceptually: all components are going to be 0 except for a single -1 in one of the distinguished positions. There are  $\lambda^* \tau = 21 \cdot 9 = 189$  of these. When combined with the 33 vectors in  $Z''$ , we should obtain a rank of 222.

```

zeroVec = Table[0, {i, 1, Length[aLst]}];

indexInTupleOf[i_, j_] := Position[aLst, {i, j}][[1]][[1]];

indexInTupleOf[2, 3]
66

aLst[[66]]
a{2,3}

```

```

tupleOfSVector[{i_, j_}] := Module[{result},
  (
    result = zeroVec;
    result[[indexInTupleOf[i, j]]] = -1;
    result
  )];

tupleOfSVector[{2, 3}][[66]]
-1

posOfMonInList[mon_, monLst_] := Position[monLst, mon][[1]][[1]];

posOfMonsInList[mons_, monLst_] :=
  Table[posOfMonInList[mons[[i]], monLst], {i, 1, Length[mons]}]

posOfTMMons = posOfMonsInList[TM, OO]
{8, 9, 10, 11, 28, 29, 30, 31, 32}

posOfLMMons = posOfMonsInList[LM, bdry]
{1, 2, 3, 4, 5, 6, 7, 8, 9, 10, 11, 72, 73, 74, 75, 76, 77, 78, 79, 80, 81}

```

**Note:** In a previous version of the paper, we used the term “special” for what we now call “distinguished.” The following function constructs the set of all distinguished (oldspeak: special) indices.



```
listOfSpecialIndices = Flatten[Table[{posOfTMMons[[i]], posOfLMMons[[j]]},
  {j, 1, Length[posOfLMMons]}, {i, 1, Length[posOfTMMons]}], 1]
{{8, 1}, {9, 1}, {10, 1}, {11, 1}, {28, 1}, {29, 1}, {30, 1}, {31, 1}, {32, 1}, {8, 2},
{9, 2}, {10, 2}, {11, 2}, {28, 2}, {29, 2}, {30, 2}, {31, 2}, {32, 2}, {8, 3}, {9, 3},
{10, 3}, {11, 3}, {28, 3}, {29, 3}, {30, 3}, {31, 3}, {32, 3}, {8, 4}, {9, 4}, {10, 4},
{11, 4}, {28, 4}, {29, 4}, {30, 4}, {31, 4}, {32, 4}, {8, 5}, {9, 5}, {10, 5}, {11, 5},
{28, 5}, {29, 5}, {30, 5}, {31, 5}, {32, 5}, {8, 6}, {9, 6}, {10, 6}, {11, 6},
{28, 6}, {29, 6}, {30, 6}, {31, 6}, {32, 6}, {8, 7}, {9, 7}, {10, 7}, {11, 7},
{28, 7}, {29, 7}, {30, 7}, {31, 7}, {32, 7}, {8, 8}, {9, 8}, {10, 8}, {11, 8},
{28, 8}, {29, 8}, {30, 8}, {31, 8}, {32, 8}, {8, 9}, {9, 9}, {10, 9}, {11, 9},
{28, 9}, {29, 9}, {30, 9}, {31, 9}, {32, 9}, {8, 10}, {9, 10}, {10, 10}, {11, 10},
{28, 10}, {29, 10}, {30, 10}, {31, 10}, {32, 10}, {8, 11}, {9, 11}, {10, 11},
{11, 11}, {28, 11}, {29, 11}, {30, 11}, {31, 11}, {32, 11}, {8, 72}, {9, 72},
{10, 72}, {11, 72}, {28, 72}, {29, 72}, {30, 72}, {31, 72}, {32, 72}, {8, 73},
{9, 73}, {10, 73}, {11, 73}, {28, 73}, {29, 73}, {30, 73}, {31, 73}, {32, 73},
{8, 74}, {9, 74}, {10, 74}, {11, 74}, {28, 74}, {29, 74}, {30, 74}, {31, 74},
{32, 74}, {8, 75}, {9, 75}, {10, 75}, {11, 75}, {28, 75}, {29, 75}, {30, 75},
{31, 75}, {32, 75}, {8, 76}, {9, 76}, {10, 76}, {11, 76}, {28, 76}, {29, 76},
{30, 76}, {31, 76}, {32, 76}, {8, 77}, {9, 77}, {10, 77}, {11, 77}, {28, 77},
{29, 77}, {30, 77}, {31, 77}, {32, 77}, {8, 78}, {9, 78}, {10, 78}, {11, 78},
{28, 78}, {29, 78}, {30, 78}, {31, 78}, {32, 78}, {8, 79}, {9, 79}, {10, 79},
{11, 79}, {28, 79}, {29, 79}, {30, 79}, {31, 79}, {32, 79}, {8, 80}, {9, 80},
{10, 80}, {11, 80}, {28, 80}, {29, 80}, {30, 80}, {31, 80}, {32, 80}, {8, 81},
{9, 81}, {10, 81}, {11, 81}, {28, 81}, {29, 81}, {30, 81}, {31, 81}, {32, 81}}
```

```
listOfSVectors = Table[tupleOfSVector[listOfSpecialIndices[[i]]],
  {i, 1, Length[listOfSpecialIndices]};
```

```
Length[listOfSVectors]
```

```
189
```

The following line should return {0}. If it does, it verifies that all of the tuples in the **listOfSVectors** are indeed tangent vectors at  $[I]$ , since they satisfy all of the tangent space relations.

```
DeleteDuplicates[Flatten[Table[allTanSpaceRelns[[i]].listOfSVectors[[j]],
  {i, 1, Length[allTanSpaceRelns]}, {j, 1, Length[listOfSVectors]}]]]
```

```
{0}
```

If the following line returns 222, it demonstrates that the set of tangent vectors  $S \cup Z''$  is linearly independent, and consequently that our ideal is generic on an elementary component of dimension 222.

```
MatrixRank[Join[listOfSVectors, zTuples]]
```

```
222
```
