# Supplementary material for: Some elementary components of the Hilbert scheme of points
Source: arXiv:1407.1440 ancillary file (2016-01-21)
Supplement: Supplementary file 5 [file case__1_6_10_10_5_0__third.pdf]

# Case (1,6,10,10,5,0) third.

This file accompanies the paper *Some Elementary Components of the Hilbert Scheme of Points*, to appear in the *Rocky Mountain Journal of Mathematics*.

Author: Mark Huibregtse

Affiliation: Skidmore College .

Email address: mhuibreg@skidmore.edu .

This is the third of three generic examples with Hilbert function (1, 6, 10, 10, 5, 0); it is presented in section 8.5.3 of the paper. As in the preceding example (section 8.5.2), some of the trailing monomials are lex-larger than some of the leading monomials, so Corollary 7.5 does not apply. On the other hand, we show by direct computation that the set of tangent vectors  $S \sim Z$  is linearly independent for sufficiently general distinguished ideals  $I$ . It turns out that the dimension of this set of vectors is 211, which accordingly (Corollary 7.7) is a lower bound on the dimension of an irreducible locus containing the point  $[I]$ . Since the dimension of the tangent space at  $[I]$  is also 211, it follows from Proposition 5.5 that  $I$  is generic.

Assign the number of variables  $n$ , the list of variables  $\{x_1, \dots, x_n\}$ , and the list of null substitutions  $\{x_1 \rightarrow 0, \dots, x_n \rightarrow 0\}$ .

```
n = 6;  
varList = Table[xi, {i, 1, n}];  
nullSubs = makeNullSubLst[varList];
```

Make the lex-segment complement order ideal for Hilbert function (1,6,10,10,5,0), and the set of boundary monomials.

```
OO = makeOrderIdeal[{1, 6, 10, 10, 5}, varList]  
{1, x1, x2, x3, x4, x5, x6, x32, x3 x4, x3 x5, x3 x6, x42, x4 x5, x4 x6, x52, x5 x6, x62, x43,  
x42 x5, x42 x6, x4 x52, x4 x5 x6, x4 x62, x53, x52 x6, x5 x62, x63, x54, x53 x6, x52 x62, x5 x63, x64}
```

```
 $\mu$  = Length[OO]
```

```
bdry = bdryMonoms[OO, varList]
```

$$\left\{ x_1^2, x_1 x_2, x_1 x_3, x_1 x_4, x_1 x_5, x_1 x_6, x_2^2, x_2 x_3, x_2 x_4, x_2 x_5, x_2 x_6, x_1 x_3^2, x_1 x_3 x_4, \right. \\ x_1 x_3 x_5, x_1 x_3 x_6, x_1 x_4^2, x_1 x_4 x_5, x_1 x_4 x_6, x_1 x_5^2, x_1 x_5 x_6, x_1 x_6^2, x_2 x_3^2, x_2 x_3 x_4, \\ x_2 x_3 x_5, x_2 x_3 x_6, x_2 x_4^2, x_2 x_4 x_5, x_2 x_4 x_6, x_2 x_5^2, x_2 x_5 x_6, x_2 x_6^2, x_3^3, x_3^2 x_4, x_3^2 x_5, \\ x_3^2 x_6, x_3 x_4^2, x_3 x_4 x_5, x_3 x_4 x_6, x_3 x_5^2, x_3 x_5 x_6, x_3 x_6^2, x_1 x_4^3, x_1 x_4^2 x_5, x_1 x_4^2 x_6, \\ x_1 x_4 x_5^2, x_1 x_4 x_5 x_6, x_1 x_4 x_6^2, x_1 x_5^3, x_1 x_5^2 x_6, x_1 x_5 x_6^2, x_1 x_6^3, x_2 x_4^3, x_2 x_4^2 x_5, x_2 x_4^2 x_6, \\ x_2 x_4 x_5^2, x_2 x_4 x_5 x_6, x_2 x_4 x_6^2, x_2 x_5^3, x_2 x_5^2 x_6, x_2 x_5 x_6^2, x_2 x_6^3, x_3 x_4^3, x_3 x_4^2 x_5, x_3 x_4^2 x_6, \\ x_3 x_4 x_5^2, x_3 x_4 x_5 x_6, x_3 x_4 x_6^2, x_3 x_5^3, x_3 x_5^2 x_6, x_3 x_5 x_6^2, x_3 x_6^3, x_4^4, x_4^3 x_5, x_4^3 x_6, x_4^2 x_5^2, \\ x_4^2 x_5 x_6, x_4^2 x_6^2, x_4 x_5^3, x_4 x_5^2 x_6, x_4 x_5 x_6^2, x_4 x_6^3, x_1 x_5^4, x_1 x_5^3 x_6, x_1 x_5^2 x_6^2, x_1 x_5 x_6^3, \\ x_1 x_6^4, x_2 x_5^4, x_2 x_5^3 x_6, x_2 x_5^2 x_6^2, x_2 x_5 x_6^3, x_2 x_6^4, x_3 x_5^4, x_3 x_5^3 x_6, x_3 x_5^2 x_6^2, x_3 x_5 x_6^3, \\ x_3 x_6^4, x_4 x_5^4, x_4 x_5^3 x_6, x_4 x_5^2 x_6^2, x_4 x_5 x_6^3, x_4 x_6^4, x_5^5, x_5^4 x_6, x_5^3 x_6^2, x_5^2 x_6^3, x_5 x_6^4, x_6^5 \}$$

```
numBdry = Length[bdry]
```

```
107
```

## Form the sets of leading and trailing monomials LM and TM

```
mins = minBdryMons[OO, bdry, varList]
```

$$\left\{ x_1^2, x_1 x_2, x_1 x_3, x_1 x_4, x_1 x_5, x_1 x_6, x_2^2, x_2 x_3, x_2 x_4, x_2 x_5, x_2 x_6, x_3^3, x_3^2 x_4, \right. \\ x_3^2 x_5, x_3^2 x_6, x_3 x_4^2, x_3 x_4 x_5, x_3 x_4 x_6, x_3 x_5^2, x_3 x_5 x_6, x_3 x_6^2, x_4^4, x_4^3 x_5, x_4^3 x_6, x_4^2 x_5^2, \\ x_4^2 x_5 x_6, x_4^2 x_6^2, x_4 x_5^3, x_4 x_5^2 x_6, x_4 x_5 x_6^2, x_4 x_6^3, x_5^5, x_5^4 x_6, x_5^3 x_6^2, x_5^2 x_6^3, x_5 x_6^4, x_6^5 \}$$

```
Length[mins]
```

```
37
```

```
LM = Join[Take[mins, 11], Take[mins, -6]]
```

$$\left\{ x_1^2, x_1 x_2, x_1 x_3, x_1 x_4, x_1 x_5, x_1 x_6, x_2^2, \right. \\ x_2 x_3, x_2 x_4, x_2 x_5, x_2 x_6, x_5^5, x_5^4 x_6, x_5^3 x_6^2, x_5^2 x_6^3, x_5 x_6^4, x_6^5 \}$$

```
λ = Length[LM]
```

```
17
```

```
maxes = maxBasisMons[OO, bdry, varList]
```

$$\left\{ x_1, x_2, x_3^2, x_3 x_4, x_3 x_5, x_3 x_6, x_4^3, x_4^2 x_5, \right. \\ x_4^2 x_6, x_4 x_5^2, x_4 x_5 x_6, x_4 x_6^2, x_5^4, x_5^3 x_6, x_5^2 x_6^2, x_5 x_6^3, x_6^4 \}$$

```
TM = Join[Take[maxes, {3, 12}]]
```

$$\left\{ x_3^2, x_3 x_4, x_3 x_5, x_3 x_6, x_4^3, x_4^2 x_5, x_4^2 x_6, x_4 x_5^2, x_4 x_5 x_6, x_4 x_6^2 \right\}$$

```
τ = Length[TM]
```

```
10
```

Randomly generate a short list of polynomials  $G$ , test for efficiency and  $\theta$ -

efficiency, and make the associated border basis of the distinguished ideal associated to the short list.

```
G = makeShortListOfIdealGenerators[LM, TM]
{ x1^2 + x3^2 + x3 x4 + x4^3 - x4^2 x5 - x3 x6 - x4^2 x6, x1 x2 - x4^3 - x3 x5 + x4 x5^2 - x3 x6 + x4^2 x6 + x4 x5 x6 + x4 x6^2,
  x1 x3 - x3^2 - x3 x5 + x4^2 x5 + x4 x5^2 - x3 x6 + x4^2 x6 + x4 x5 x6 - x4 x6^2,
  x1 x4 - x3 x4 - x3 x5 + x4^2 x5 - x4 x5^2 - x3 x6 + x4^2 x6 - x4 x5 x6 + x4 x6^2,
  -x3^2 - x3 x4 + x4^3 + x1 x5 + x4^2 x5 + x4^2 x6 + x4 x6^2, -x3^2 + x4^2 x5 + x4 x5^2 + x1 x6 + x3 x6,
  x2^2 + x3 x4 + x4^3 + x3 x5 + x4^2 x5 + x4 x5^2 + x3 x6 + x4^2 x6 + x4 x6^2, x2 x3 - x4^3 + x3 x5 - x4 x5^2 + x4^2 x6 - x4 x6^2,
  x3^2 + x2 x4 - x4^2 x5 - x4 x5^2 + x4^2 x6 - x4 x5 x6, x2 x5 - x3 x5 - x4^2 x5 - x4 x5^2 + x3 x6 - x4^2 x6 - x4 x5 x6,
  -x3^2 - x3 x4 - x3 x5 - x4^2 x5 - x4 x5^2 + x2 x6 + x3 x6 + x4^2 x6 - x4 x5 x6,
  x3^2 + x3 x4 - x4^3 + x3 x5 + x4^2 x5 - x4 x5^2 + x3^2 + x3 x6 + x4^2 x6,
  -x4^3 - x4^2 x5 + x4 x5^2 + x3 x6 + x4^2 x6 - x4 x5 x6 + x4^2 x6,
  x3^2 + x4^3 - x3 x5 - x4^2 x5 - x4 x5^2 - x4^2 x6 + x4 x5 x6 + x3^2 x6^2,
  x3^2 + x3 x4 - x4^3 - x3 x5 - x4^2 x5 - x4 x5^2 + x4^2 x6 + x4 x6^2 + x5^2 x6^3,
  -x3^2 + x3 x4 + x4^2 x5 + x4 x5 x6 + x4 x6^2 + x5 x6^4, -x3^2 - x4^2 x5 + x4 x5^2 + x3 x6 + x4^2 x6 - x4 x5 x6 - x4 x6^2 + x5^2 x6^5 }
```

This example was generated on 3/06/2014 -- it is generic. It is efficient but not theta-efficient. The dimension of the component is 211. LOVELY -- we have three different components associated to the basis set (1,6,10,10,5). Very nice example.

```
(* G = { x1^2 - x3^2 - x3 x4 - x4^3 - x3 x5 - x4^2 x5 + x4 x5^2 - x3 x6 - x4^2 x6 + x4 x5 x6 - x4 x6^2,
  x1 x2 + x3^2 + x3 x4 + x4^3 - x3 x5 - x4^2 x5 - x4 x5^2 + x4^2 x6 + x4 x5 x6 - x4 x6^2,
  x1 x3 - x4^3 + x3 x5 - x4 x5^2 + x3 x6 - x4^2 x6 - x4 x5 x6,
  -x3^2 + x1 x4 + x3 x4 + x3 x5 + x3 x6 - x4 x5 x6 + x4 x6^2, x3^2 - x3 x4 - x4^3 + x1 x5 + x3 x5 + x4^2 x5 + x4 x5^2 - x4 x6^2,
  x3 x4 + x4^3 + x4^2 x5 - x4 x5^2 + x1 x6 - x3 x6 - x4^2 x6 + x4 x6^2,
  x2^2 + x3 x4 - x4^3 - x4^2 x5 + x4 x5^2 + x4^2 x6 - x4 x5 x6, x2 x3 + x3^2 - x3 x4 - x3 x6 - x4 x5 x6 - x4 x6^2,
  x2 x4 + x3 x4 - x4^3 - x4^2 x5 - x4 x5^2 - x3 x6 + x4^2 x6 + x4 x5 x6 + x4 x6^2,
  x3^2 - x3 x4 + x4^3 + x2 x5 - x4^2 x5 + x4 x5^2 - x4 x5 x6 + x4 x6^2, -x3^2 - x4^2 x5 + x4 x5^2 + x2 x6 + x3 x6 - x4^2 x6 + x4 x5 x6,
  -x3 x4 - x4^3 + x4^2 x5 + x4 x5^2 + x3 x6 + x4^2 x6 - x4 x5 x6, x3 x4 + x4^3 + x4^2 x5 - x4 x5^2 - x4^2 x6 + x4 x5^2 x6,
  -x3^2 + x4^3 + x3 x5 - x4^2 x5 + x3 x6 - x4 x5 x6 + x5^2 x6^3, x4^3 + x3 x5 + x4^2 x5 - x3 x6 + x4 x5 x6 - x4 x6^2 + x5^2 x6^3,
  x3^2 - x4^3 - x3 x5 + x4^2 x5 - x4 x5^2 - x3 x6 + x4^2 x6 - x4 x5 x6 + x5 x6^4,
  -x3 x4 - x3 x5 - x4^2 x5 - x4^2 x6 - x4 x5 x6 + x5^2 x6^5 }; *)
```

```
Length[G]
```

```
17
```

```
isEfficient[G, LM, bdry, varList]
```

```
True
```

```
isThetaEfficient[G, LM, TM, bdry, varList, verbose = True]
```

```

Condition 1 of Proposition 3.1 is True.
(numProds = 102) < (numQ = 105)
The map  $\vartheta$  is not surjective.
False

borBasis = makeBorderBasisOfI[G, bdry, LM];

```

## Find the tangent space relations and the dimension of the tangent space at $[I]$

```

{aLst, allTanSpaceRelns} = makeTanSpaceRelns[borBasis, OO, bdry, varList];

tanSpaceDim[Length[aLst], allTanSpaceRelns]
211

```

As shown in Section 8.5.3 of the paper, the set of tangent vectors  $S \cup Z''$  has cardinality 211. If we can show that these vectors are linearly independent at  $[I]$ , then we will know that the dimension of the locus  $F(U)$  is  $\geq 211$ ; whence,  $I$  is generic and  $[I]$  is smooth on an elementary component of dimension 211. In the next section of the notebook, we compute the tuples  $(a_{ij})$  corresponding to the tangent vectors in  $S \cup Z''$  and show by direct computation that they are linearly independent. We need to do this computationally, since we don't have any general theorems stating when  $S \cup Z''$  is linearly independent.

The tuples are produced by following the "recipe" given in equation (22) of section 6.2 of the paper.

---

## Create explicit tuples corresponding to the vectors in $S \cup Z''$

### $x_\alpha$ -translations (or partial with respect to $x_\alpha$ )

The following function makes the tuples corresponding to the  $n$  tangent vectors given by translating in the  $x_1, \dots, x_n$ -directions.

```

makeTranslationVector[var_] := Flatten[
  Table[coeffOfTerm[ reducePoly[D[borBasis[[j]], var], bdry, borBasis, varList] ,
    OO[[i]] , varList], {j, 1, numBdry}, {i, 1,  $\mu$ }, 1];

x1trans = makeTranslationVector[x1];

Length[x1trans]
3424

numBdry *  $\mu$ 
3424

```

```

x2trans = makeTranslationVector[x2];
x3trans = makeTranslationVector[x3];
x4trans = makeTranslationVector[x4];
x5trans = makeTranslationVector[x5];
x6trans = makeTranslationVector[x6];

```

Executing the following cell for **x1trans** through **x6trans** will demonstrate that these tuples are indeed tangent vectors at  $[I]$ , since they satisfy all of the tangent space relations. (The result should be  $\{0\}$ .)

```

DeleteDuplicates[
  Table[allTanSpaceReIns[[i]].x4trans, {i, 1, Length[allTanSpaceReIns]}]]
{0}

MatrixRank[transVectors = {x1trans, x2trans, x3trans, x4trans, x5trans, x6trans}]

```

6

## Now we need to construct the remaining tangent vectors in $Z$ .

These tangent vectors correspond to the isomorphisms defined by the replacements  $(x_\alpha \rightarrow x_\alpha + m_{\{\alpha, \delta\}})$ . These are obtained by taking the partial of each member of the border basis with respect to  $x_\alpha$  and then multiplying by  $m_{\{\alpha, \delta\}}$  before taking the coefficients modulo  $I$ .

To reduce modulo  $I$ , we will use the function **reducePoly**. Because of the way the function **reducePoly** is coded, we will have to multiply by the variables appearing in  $m_{\{\alpha, \delta\}}$  one-by-one, reducing as we go. So the monomials will be entered as lists of variables which multiply to yield the monomial.

The inputs to the following function are: poly = one of the elements of the border basis; var =  $x_i$  -- the variable in the substitution  $x_i \rightarrow x_i + m$ ; and mon, the monomial  $m$  in the form of a list of the variables that constitute  $m$ : for example,  $m = x_2 x_3$  is entered as the list  $\{x_2, x_3\}$ . The output is the partial derivative of poly with respect to the given variable var multiplied by the given monomial mon, and then reduced modulo  $I$  (which results in a linear combination of the basis monomials).

```

parDerivTimesMonom[poly_, var_, mon_] := Module[{curVar, monDeg, result, i},
  (
    monDeg = Length[mon];
    result = reducePoly[D[poly, var], bdry, borBasis, varList];
    For[i = 1, i ≤ monDeg, i++,
      (
        curVar = mon[[i]];
        result = reducePoly[result * curVar, bdry, borBasis, varList];
      )];
    result
  )];

makeSubstitutionVector[var_, mon_] :=
  Flatten[Table[coeffOfTerm[ parDerivTimesMonom[borBasis[[j]], var, mon] ,
    OO[[i]], varList ], {j, 1, numBdry}, {i, 1, μ}], 1];

sub14 = makeSubstitutionVector[x1, {x4}];
sub15 = makeSubstitutionVector[x1, {x5}];
sub16 = makeSubstitutionVector[x1, {x6}];
sub155 = makeSubstitutionVector[x1, {x5, x5}];
sub156 = makeSubstitutionVector[x1, {x5, x6}];
sub166 = makeSubstitutionVector[x1, {x6, x6}];
sub1555 = makeSubstitutionVector[x1, {x5, x5, x5}];
sub1556 = makeSubstitutionVector[x1, {x5, x5, x6}];
sub1566 = makeSubstitutionVector[x1, {x5, x6, x6}];
sub1666 = makeSubstitutionVector[x1, {x6, x6, x6}];
sub24 = makeSubstitutionVector[x2, {x4}];
sub25 = makeSubstitutionVector[x2, {x5}];
sub26 = makeSubstitutionVector[x2, {x6}];
sub255 = makeSubstitutionVector[x2, {x5, x5}];
sub256 = makeSubstitutionVector[x2, {x5, x6}];
sub266 = makeSubstitutionVector[x2, {x6, x6}];
sub2555 = makeSubstitutionVector[x2, {x5, x5, x5}];
sub2556 = makeSubstitutionVector[x2, {x5, x5, x6}];
sub2566 = makeSubstitutionVector[x2, {x5, x6, x6}];

```

```

sub2666 = makeSubstitutionVector[x2, {x6, x6, x6}] ;
sub34 = makeSubstitutionVector[x3, {x4}] ;
sub35 = makeSubstitutionVector[x3, {x5}] ;
sub36 = makeSubstitutionVector[x3, {x6}] ;
sub355 = makeSubstitutionVector[x3, {x5, x5}] ;
sub356 = makeSubstitutionVector[x3, {x5, x6}] ;
sub366 = makeSubstitutionVector[x3, {x6, x6}] ;
sub3555 = makeSubstitutionVector[x3, {x5, x5, x5}] ;
sub3556 = makeSubstitutionVector[x3, {x5, x5, x6}] ;
sub3566 = makeSubstitutionVector[x3, {x5, x6, x6}] ;
sub3666 = makeSubstitutionVector[x3, {x6, x6, x6}] ;
sub45 = makeSubstitutionVector[x4, {x5}] ;
sub46 = makeSubstitutionVector[x4, {x6}] ;
sub455 = makeSubstitutionVector[x4, {x5, x5}] ;
sub456 = makeSubstitutionVector[x4, {x5, x6}] ;
sub466 = makeSubstitutionVector[x4, {x6, x6}] ;
MatrixRank[
  zTuples = Join[transVectors, {sub14, sub15, sub16, sub155, sub156, sub166, sub1555,
    sub1556, sub1566, sub1666, sub24, sub25, sub26, sub255, sub256, sub266,
    sub2555, sub2556, sub2566, sub2666, sub34, sub35, sub36, sub355, sub356, sub366,
    sub3555, sub3556, sub3566, sub3666, sub45, sub46, sub455, sub456, sub466}]]
41

```

As above, the following line can be executed for any of the tuples in the preceding list to verify that it (the chosen tuple) is indeed a tangent vector at [/].

```

DeleteDuplicates[
  Table[allTanSpaceReIns[[i]].sub3666, {i, 1, Length[allTanSpaceReIns]}]]
{0}

```

Now we create the tuples of the tangent vectors that lie in  $S$ , the tangent vectors that correspond to tweaking the coefficients of the short list of generators  $G$ .

This is easy to do, at least conceptually: all components are going to be 0 except for a single -1 in one of the special positions. There are  $\lambda^* \tau = 17 \cdot 10 = 170$  of these. When combined with the 41 vectors in  $Z$ , we should obtain a rank of 211.

```

zeroVec = Table[0, {i, 1, Length[aLst]}}];

indexInTupleOf[i_, j_] := Position[aLst, {i, j}][[1]][[1]];

indexInTupleOf[2, 3]
66

aLst[[66]]
a{2,3}

tupleOfSVector[{i_, j_}] := Module[{result},
  (
    result = zeroVec;
    result[[indexInTupleOf[i, j]]] = -1;
    result
  )];

tupleOfSVector[{2, 3}][[66]]
-1

posOfMonInList[mon_, monLst_] := Position[monLst, mon][[1]][[1]];

posOfMonsInList[mons_, monLst_] :=
  Table[posOfMonInList[mons[[i]], monLst], {i, 1, Length[mons]}]

posOfTMMons = posOfMonsInList[TM, OO]
{8, 9, 10, 11, 18, 19, 20, 21, 22, 23}

posOfLMMons = posOfMonsInList[LM, bdry]
{1, 2, 3, 4, 5, 6, 7, 8, 9, 10, 11, 102, 103, 104, 105, 106, 107}

```

**Note:** In a previous version of the paper, we used the term “special” for what we now call “distinguished.” The following function constructs the set of all distinguished (oldspeak: special) indices.



```
listOfSpecialIndices = Flatten[Table[{posOfTMMons[[i]], posOfLMMons[[j]]},
  {j, 1, Length[posOfLMMons]}, {i, 1, Length[posOfTMMons]}], 1]
{{8, 1}, {9, 1}, {10, 1}, {11, 1}, {18, 1}, {19, 1}, {20, 1}, {21, 1}, {22, 1},
{23, 1}, {8, 2}, {9, 2}, {10, 2}, {11, 2}, {18, 2}, {19, 2}, {20, 2}, {21, 2},
{22, 2}, {23, 2}, {8, 3}, {9, 3}, {10, 3}, {11, 3}, {18, 3}, {19, 3}, {20, 3},
{21, 3}, {22, 3}, {23, 3}, {8, 4}, {9, 4}, {10, 4}, {11, 4}, {18, 4}, {19, 4},
{20, 4}, {21, 4}, {22, 4}, {23, 4}, {8, 5}, {9, 5}, {10, 5}, {11, 5}, {18, 5},
{19, 5}, {20, 5}, {21, 5}, {22, 5}, {23, 5}, {8, 6}, {9, 6}, {10, 6}, {11, 6},
{18, 6}, {19, 6}, {20, 6}, {21, 6}, {22, 6}, {23, 6}, {8, 7}, {9, 7}, {10, 7},
{11, 7}, {18, 7}, {19, 7}, {20, 7}, {21, 7}, {22, 7}, {23, 7}, {8, 8}, {9, 8},
{10, 8}, {11, 8}, {18, 8}, {19, 8}, {20, 8}, {21, 8}, {22, 8}, {23, 8}, {8, 9},
{9, 9}, {10, 9}, {11, 9}, {18, 9}, {19, 9}, {20, 9}, {21, 9}, {22, 9}, {23, 9},
{8, 10}, {9, 10}, {10, 10}, {11, 10}, {18, 10}, {19, 10}, {20, 10}, {21, 10},
{22, 10}, {23, 10}, {8, 11}, {9, 11}, {10, 11}, {11, 11}, {18, 11}, {19, 11},
{20, 11}, {21, 11}, {22, 11}, {23, 11}, {8, 102}, {9, 102}, {10, 102}, {11, 102},
{18, 102}, {19, 102}, {20, 102}, {21, 102}, {22, 102}, {23, 102}, {8, 103},
{9, 103}, {10, 103}, {11, 103}, {18, 103}, {19, 103}, {20, 103}, {21, 103},
{22, 103}, {23, 103}, {8, 104}, {9, 104}, {10, 104}, {11, 104}, {18, 104},
{19, 104}, {20, 104}, {21, 104}, {22, 104}, {23, 104}, {8, 105}, {9, 105},
{10, 105}, {11, 105}, {18, 105}, {19, 105}, {20, 105}, {21, 105}, {22, 105},
{23, 105}, {8, 106}, {9, 106}, {10, 106}, {11, 106}, {18, 106}, {19, 106},
{20, 106}, {21, 106}, {22, 106}, {23, 106}, {8, 107}, {9, 107}, {10, 107},
{11, 107}, {18, 107}, {19, 107}, {20, 107}, {21, 107}, {22, 107}, {23, 107}}
```

```
listOfSVectors = Table[tupleOfSVector[listOfSpecialIndices[[i]]],
  {i, 1, Length[listOfSpecialIndices]}];
```

```
Length[listOfSVectors]
```

```
170
```

The following line should return {0}. If it does, it verifies that all of the tuples in the **listOfSVectors** are indeed tangent vectors at  $[/]$ , since they satisfy all of the tangent space relations.

```
DeleteDuplicates[Flatten[Table[allTanSpaceRelns[[i]].listOfSVectors[[j]],
  {i, 1, Length[allTanSpaceRelns]}, {j, 1, Length[listOfSVectors]}]]]
```

```
{0}
```

If the following line returns 211, it demonstrates that the set of tangent vectors  $S \cup Z''$  is linearly independent, and consequently that our ideal is generic on an elementary component of dimension 211.

```
MatrixRank[Join[listOfSVectors, zTuples]]
```

```
211
```
