# Supplementary material for: Some elementary components of the Hilbert scheme of points
Source: arXiv:1407.1440 ancillary file (2016-01-21)
Supplement: Supplementary file 6 [file case__1_6_21_10_15_0_.pdf]

# Case (1,6,21,10,15,0).

This file accompanies the paper *Some Elementary Components of the Hilbert Scheme of Points*, to appear in the *Rocky Mountain Journal of Mathematics*.

Author: Mark Huibregtse

Affiliation: Skidmore College .

Email address: mhuibreg@skidmore.edu .

This notebook contains the details of the example presented in Section 8.4 of the paper.

Assign the number of variables  $n$ , the list of variables  $\{x_1, \dots, x_n\}$ , and the list of null substitutions  $\{x_1 \rightarrow 0, \dots, x_n \rightarrow 0\}$ .

```
n = 6;  
varList = Table[xi, {i, 1, n}];  
nullSubs = makeNullSubLst[varList];
```

Make the lex-segment complement order ideal for Hilbert function (1,6,21,10,15,0) and the set of boundary monomials:

```
OO = makeOrderIdeal[{1, 6, 21, 10, 15}, varList]  
{1, x1, x2, x3, x4, x5, x6, x12, x1 x2, x1 x3, x1 x4, x1 x5, x1 x6, x22, x2 x3,  
x2 x4, x2 x5, x2 x6, x32, x3 x4, x3 x5, x3 x6, x42, x4 x5, x4 x6, x52, x5 x6, x62, x43,  
x42 x5, x42 x6, x4 x52, x4 x5 x6, x4 x62, x53, x52 x6, x5 x62, x63, x44, x43 x5, x43 x6, x42 x52,  
x42 x5 x6, x42 x62, x4 x53, x4 x52 x6, x4 x5 x62, x4 x63, x54, x53 x6, x52 x62, x5 x63, x64}  
  
μ = Length[OO]  
53  
  
bdry = bdryMonoms[OO, varList];  
numBdry = Length[bdry]  
142
```

Form the sets of leading and trailing monomials LM and TM

```
mins = minBdryMons[00, bdry, varList]
```

$$\{x_1^3, x_1^2 x_2, x_1^2 x_3, x_1^2 x_4, x_1^2 x_5, x_1^2 x_6, x_1 x_2^2, x_1 x_2 x_3, x_1 x_2 x_4, x_1 x_2 x_5, x_1 x_2 x_6, x_1 x_3^2, x_1 x_3 x_4, x_1 x_3 x_5, x_1 x_3 x_6, x_1 x_4^2, x_1 x_4 x_5, x_1 x_4 x_6, x_1 x_5^2, x_1 x_5 x_6, x_1 x_6^2, x_2^3, x_2^2 x_3, x_2^2 x_4, x_2^2 x_5, x_2^2 x_6, x_2 x_3^2, x_2 x_3 x_4, x_2 x_3 x_5, x_2 x_3 x_6, x_2 x_4^2, x_2 x_4 x_5, x_2 x_4 x_6, x_2 x_5^2, x_2 x_5 x_6, x_2 x_6^2, x_3^3, x_3^2 x_4, x_3^2 x_5, x_3^2 x_6, x_3 x_4^2, x_3 x_4 x_5, x_3 x_4 x_6, x_3 x_5^2, x_3 x_5 x_6, x_3 x_6^2, x_4^3, x_4^2 x_5, x_4^2 x_6, x_4 x_5^2, x_4 x_5 x_6, x_4 x_6^2, x_5^3, x_5^2 x_6, x_5 x_6^2, x_6^3, x_6^2 x_5, x_6 x_5^2, x_6 x_5^3\}$$

```
LM = Take[mins, 46]
```

$$\{x_1^3, x_1^2 x_2, x_1^2 x_3, x_1^2 x_4, x_1^2 x_5, x_1^2 x_6, x_1 x_2^2, x_1 x_2 x_3, x_1 x_2 x_4, x_1 x_2 x_5, x_1 x_2 x_6, x_1 x_3^2, x_1 x_3 x_4, x_1 x_3 x_5, x_1 x_3 x_6, x_1 x_4^2, x_1 x_4 x_5, x_1 x_4 x_6, x_1 x_5^2, x_1 x_5 x_6, x_1 x_6^2, x_2^3, x_2^2 x_3, x_2^2 x_4, x_2^2 x_5, x_2^2 x_6, x_2 x_3^2, x_2 x_3 x_4, x_2 x_3 x_5, x_2 x_3 x_6, x_2 x_4^2, x_2 x_4 x_5, x_2 x_4 x_6, x_2 x_5^2, x_2 x_5 x_6, x_2 x_6^2, x_3^3, x_3^2 x_4, x_3^2 x_5, x_3^2 x_6, x_3 x_4^2, x_3 x_4 x_5, x_3 x_4 x_6, x_3 x_5^2, x_3 x_5 x_6, x_3 x_6^2\}$$
$$\lambda = \text{Length}[\text{LM}]$$

46

```
maxes = maxBasisMons[00, bdry, varList]
```

$$\{x_1^2, x_1 x_2, x_1 x_3, x_1 x_4, x_1 x_5, x_1 x_6, x_2^2, x_2 x_3, x_2 x_4, x_2 x_5, x_2 x_6, x_3^2, x_3 x_4, x_3 x_5, x_3 x_6, x_4^2, \\ x_4^3 x_5, x_4^3 x_6, x_4^2 x_5^2, x_4^2 x_5 x_6, x_4^2 x_6^2, x_4 x_5^3, x_4 x_5^2 x_6, x_4 x_5 x_6^2, x_4 x_6^3, x_5^4, x_5^3 x_6, x_5^2 x_6^2, x_5 x_6^3, x_6^4\}$$

```
TM = Take[maxes, -15]
```

$$\{x_4^4, x_4^3 x_5, x_4^3 x_6, x_4^2 x_5^2, x_4^2 x_5 x_6, x_4^2 x_6^2, \\ x_4 x_5^3, x_4 x_5^2 x_6, x_4 x_5 x_6^2, x_4 x_6^3, x_5^4, x_5^3 x_6, x_5^2 x_6^2, x_5 x_6^3, x_6^4\}$$
$$\tau = \text{Length}[\text{TM}]$$

15

Randomly generate a short list of polynomials  $G$ , test for efficiency and  $\theta$ -efficiency, and make the associated border basis of the distinguished ideal associated to the short list.

A previously-generated example that “works” is in the cell following the next cell that generates a new example at random.

```
G = makeShortListOfIdealGenerators[LM, TM];
```

This example that “works” was generated on 8/09/2013.

$$\begin{aligned} (*\text{gensOfI} = & \{ \mathbf{x}_1^3 + \mathbf{x}_4^4 - \mathbf{x}_2^4, \mathbf{x}_5^2 - \mathbf{x}_5^4 + \mathbf{x}_4^3, \mathbf{x}_6 + \mathbf{x}_4^2, \mathbf{x}_5, \mathbf{x}_6 - \mathbf{x}_5^3, \mathbf{x}_6 - \mathbf{x}_4^2, \mathbf{x}_6^2 - \mathbf{x}_6^4, \\ & \mathbf{x}_1^2, \mathbf{x}_2 - \mathbf{x}_4^3, \mathbf{x}_5 - \mathbf{x}_4^2, \mathbf{x}_5^2 + \mathbf{x}_5^4 - \mathbf{x}_3^3, \mathbf{x}_6 + \mathbf{x}_4^2, \mathbf{x}_5, \mathbf{x}_6 - \mathbf{x}_4, \mathbf{x}_5^2, \mathbf{x}_6 + \mathbf{x}_5^3, \mathbf{x}_6 + \mathbf{x}_4^2, \mathbf{x}_6^2 + \mathbf{x}_4, \mathbf{x}_5, \mathbf{x}_6^2 + \mathbf{x}_5^2, \mathbf{x}_6^2 - \mathbf{x}_5, \mathbf{x}_6^3 + \mathbf{x}_6^4, \\ & \mathbf{x}_1^2, \mathbf{x}_3 - \mathbf{x}_4^4 + \mathbf{x}_4^2, \mathbf{x}_5^2 - \mathbf{x}_4, \mathbf{x}_5^3 - \mathbf{x}_4^4 - \mathbf{x}_4^2, \mathbf{x}_5, \mathbf{x}_6 + \mathbf{x}_4, \mathbf{x}_5^2, \mathbf{x}_6 - \mathbf{x}_5^3, \mathbf{x}_6 - \mathbf{x}_4^2, \mathbf{x}_6^2 - \mathbf{x}_5^2, \mathbf{x}_6^2 - \mathbf{x}_4, \mathbf{x}_6^3 - \mathbf{x}_6^4, \end{aligned}$$

$$\begin{aligned}
& x_1^2 x_4 + x_4^4 - x_4^3 x_5 + x_4^2 x_5^2 + x_4 x_5^3 - x_5^4 + x_4^3 x_6 - x_4 x_5^2 x_6 - x_4^2 x_6^2 - x_5^2 x_6^2 - x_5 x_6^3, \\
& x_1^2 x_5 + x_4^3 x_5 - x_4^2 x_5^2 + x_4 x_5^3 + x_5^4 - x_5^3 x_6 + x_4^2 x_6^2 - x_4 x_5^2 x_6^2 - x_4 x_6^3 + x_4^4, \\
& x_4 x_5^3 + x_5^4 + x_1^2 x_6 - x_4^2 x_5 x_6 + x_5^3 x_6 - x_4 x_5^2 x_6^2 - x_4^2 x_6^2 - x_4 x_6^3 + x_5^3 x_6^2 + x_6^4, \\
& x_1 x_2^2 - x_4^4 + x_4^3 x_5^2 - x_5^4 + x_4^3 x_6 - x_5^3 x_6 + x_4^2 x_6^2 + x_4 x_5^2 x_6^2 + x_5^2 x_6^2 + x_5^3 x_6^2, \\
& x_1 x_2 x_3 - x_4^4 + x_4^3 x_5^2 - x_4 x_5^3 - x_4^3 x_6 - x_5^2 x_6^2 + x_5 x_6^3 - x_4 x_5^2 x_6^2 + x_5^2 x_6^2 + x_5^3 x_6^2, \\
& x_1 x_2 x_4 - x_4^4 - x_4^3 x_5^2 + x_4^2 x_5^3 - x_4 x_5^4 - x_4^3 x_6 - x_5^4 - x_4^2 x_6^2 + x_5 x_6^3 - x_4 x_5^2 x_6^2 + x_5^2 x_6^2 + x_5^3 x_6^2 + x_5^4 - \\
& \quad x_5^2 x_6^2 + x_5 x_6^3 - x_6^4, -x_4^4 + x_1 x_2 x_5 + x_4^2 x_5^2 - x_4 x_5^3 - x_4^3 x_5^4 + x_4^2 x_6^2 + x_4 x_5^2 x_6^2 + x_5^2 x_6^2 + x_5^3 x_6^2 + x_5^4 - x_6^4, \\
& x_4^4 - x_4^3 x_5 - x_4 x_5^3 + x_5^4 + x_1 x_2 x_6 + x_4^3 x_6 + x_4^2 x_5^2 x_6 + x_5 x_6^3 - x_4^2 x_6^2 + x_4 x_5^2 x_6^2 + x_5^2 x_6^2 + x_5^3 x_6^2, \\
& x_1 x_2^3 - x_4^4 + x_4^3 x_5^2 + x_4^2 x_5^3 - x_4 x_5^4 - x_4^3 x_6 + x_4^2 x_5^2 x_6 + x_5 x_6^3 - x_4 x_5^2 x_6^2 + x_5^2 x_6^2 + x_5^3 x_6^2, \\
& x_1 x_3 x_4 - x_4^3 x_5 + x_4^2 x_5^2 + x_4 x_5^3 - x_5^4 - x_4^2 x_6^2 + x_5 x_6^3 + x_4 x_5^2 x_6^2 - x_4 x_6^3 + x_5^3 x_6^2 + x_6^4, \\
& -x_4^4 + x_1 x_3 x_5 + x_4^2 x_5^2 + x_4 x_5^3 - x_5^4 - x_4^2 x_6^2 + x_5 x_6^3 + x_4 x_5^2 x_6^2 + x_5^2 x_6^2 + x_5^3 x_6^2 - x_6^4, \\
& x_4^4 + x_4^3 x_5 - x_4 x_5^3 + x_5^4 + x_1 x_3 x_6 + x_4^3 x_6 + x_4^2 x_5^2 x_6 + x_5 x_6^3 - x_4^2 x_6^2 + x_4 x_5^2 x_6^2 + x_5^2 x_6^2 + x_5^3 x_6^2 + x_5^4 - x_6^4, \\
& x_1 x_2^4 + x_4^4 - x_4^3 x_5^2 + x_4^2 x_5^3 + x_4 x_5^4 - x_4^3 x_6 - x_5^2 x_6^2 + x_5 x_6^3 - x_4 x_5^2 x_6^2 + x_5^2 x_6^2 + x_5^3 x_6^2, \\
& x_4^4 + x_1 x_4 x_5 + x_4^3 x_5^2 + x_4^2 x_5^3 + x_4 x_5^4 - x_4^3 x_6 - x_5^2 x_6^2 + x_5 x_6^3 - x_4 x_5^2 x_6^2 + x_5^2 x_6^2 + x_5^3 x_6^2 + x_5^4, \\
& x_4^4 + x_4^3 x_5 + x_4 x_5^3 + x_5^4 + x_1 x_4 x_6 + x_4^3 x_6 + x_4^2 x_5^2 x_6 + x_5 x_6^3 - x_4^2 x_6^2 + x_4 x_5^2 x_6^2 + x_5^2 x_6^2 + x_5^3 x_6^2 - x_6^4, \\
& -x_4^4 - x_4^3 x_5 + x_1 x_5^2 + x_4^2 x_5^3 - x_5^4 - x_4^2 x_6^2 + x_5 x_6^3 + x_4 x_5^2 x_6^2 - x_4 x_6^3 + x_5^3 x_6^2 + x_6^4, \\
& -x_4^4 + x_4^2 x_5^2 - x_4 x_5^3 + x_1 x_5 x_6 + x_4^2 x_5^2 x_6 + x_5^2 x_6^2 - x_4 x_6^3 - x_5^3 x_6^2 + x_6^4, \\
& x_4^3 x_5 + x_4^2 x_5^2 + x_5^4 + x_4^3 x_6 - x_4 x_5^2 x_6^2 + x_5^2 x_6^2 + x_5^3 x_6^2, \\
& x_2^3 - x_4^3 x_5 - x_4^2 x_5^2 + x_5^4 - x_4^2 x_5^3 - x_4 x_5^4 - x_4^2 x_6^2 + x_5 x_6^3 - x_4 x_5^2 x_6^2 + x_5^2 x_6^2 - x_6^4, \\
& x_2^2 x_3 + x_4^4 - x_4^3 x_5 - x_4^2 x_5^2 - x_4 x_5^3 - x_5^4 + x_4^2 x_6^2 + x_5 x_6^3 - x_4 x_5^2 x_6^2 + x_5^2 x_6^2 + x_5^3 x_6^2 - x_6^4, \\
& x_2^2 x_4 - x_4^3 x_5 + x_4^2 x_5^2 - x_4 x_5^3 - x_4^2 x_6^2 + x_5 x_6^3 - x_4 x_5^2 x_6^2 + x_5^2 x_6^2 + x_5^3 x_6^2, \\
& x_2^2 x_5 + x_4^3 x_5 + x_4 x_5^3 - x_5^4 + x_4^2 x_6^2 + x_5 x_6^3 - x_4 x_5^2 x_6^2 + x_5^2 x_6^2 + x_5^3 x_6^2, \\
& -x_4^4 + x_4^3 x_5 + x_5^4 + x_2^2 x_6 + x_4^2 x_6^2 - x_4 x_5^2 x_6^2 + x_5^2 x_6^2 + x_5^3 x_6^2 - x_6^4, \\
& x_2 x_3^2 + x_4^4 - x_4^3 x_5^2 + x_4^2 x_5^3 - x_4 x_5^4 + x_4^2 x_6^2 + x_5 x_6^3 - x_4 x_5^2 x_6^2 + x_5^2 x_6^2 + x_5^3 x_6^2, \\
& x_2 x_3 x_4 - x_4^3 x_5 + x_4^2 x_5^2 - x_4 x_5^3 - x_4^2 x_6^2 + x_5 x_6^3 - x_4 x_5^2 x_6^2 + x_5^2 x_6^2 + x_5^3 x_6^2, \\
& x_4^4 + x_2 x_3 x_5 - x_4^3 x_5^2 + x_4^2 x_5^3 - x_4 x_5^4 + x_4^2 x_6^2 + x_5 x_6^3 - x_4 x_5^2 x_6^2 + x_5^2 x_6^2 + x_5^3 x_6^2, \\
& -x_4^4 + x_4^3 x_5 + x_4^2 x_5^2 + x_2 x_3 x_6 - x_4^2 x_6^2 + x_5 x_6^3 - x_4 x_5^2 x_6^2 + x_5^2 x_6^2 + x_5^3 x_6^2 - x_6^4, \\
& x_2 x_4^2 - x_4^4 + x_4^3 x_5^2 - x_5^4 + x_4^2 x_6^2 + x_5 x_6^3 - x_4 x_5^2 x_6^2 + x_5^2 x_6^2 + x_5^3 x_6^2 - x_6^4, \\
& x_2 x_4 x_5 - x_4^2 x_5^2 + x_4 x_5^3 - x_4^2 x_6^2 + x_5 x_6^3 - x_4 x_5^2 x_6^2 + x_5^2 x_6^2 + x_5^3 x_6^2, \\
& x_4^4 + x_4^3 x_5 + x_4 x_5^3 + x_2 x_4 x_6 - x_4^3 x_6^2 - x_4^2 x_5^2 x_6 + x_5 x_6^3 - x_4 x_5^2 x_6^2 + x_5^2 x_6^2 + x_5^3 x_6^2, \\
& x_2 x_5^2 - x_4^3 x_5^2 - x_4^2 x_5^3 + x_4 x_5^4 - x_4^2 x_6^2 + x_5 x_6^3 - x_4 x_5^2 x_6^2 + x_5^2 x_6^2 + x_5^3 x_6^2, \\
& -x_4^3 x_5 - x_4^2 x_5^2 + x_4 x_5^3 + x_2 x_5 x_6 - x_4^2 x_6^2 + x_5 x_6^3 - x_4 x_5^2 x_6^2 + x_5^2 x_6^2 + x_5^3 x_6^2, \\
& x_4^4 + x_4^3 x_5 + x_4^2 x_5^2 - x_4 x_5^3 + x_2 x_5^2 x_6 + x_4^2 x_6^2 + x_5 x_6^3 - x_4 x_5^2 x_6^2 + x_5^2 x_6^2 - x_5^3 x_6^2, \\
& x_3^3 - x_4^3 x_5^2 - x_4^2 x_5^3 + x_4 x_6^2 - x_4^2 x_5 x_6 + x_5 x_6^3 - x_4 x_5^2 x_6^2 + x_5^2 x_6^2 + x_5^3 x_6^2, \\
& x_2^3 x_4 + x_4^4 - x_4^3 x_5 + x_4^2 x_5^2 + x_4 x_5^3 - x_5^4 - x_4^2 x_6^2 + x_5 x_6^3 - x_4 x_5^2 x_6^2 + x_5^2 x_6^2 + x_5^3 x_6^2 - x_6^4, \\
& x_2^3 x_5 - x_4^3 x_5 + x_4^2 x_5^2 + x_4 x_5^3 + x_5^4 - x_4^2 x_6^2 + x_5 x_6^3 - x_4 x_5^2 x_6^2 + x_5^2 x_6^2 + x_5^3 x_6^2 - x_6^4, \\
& -x_4^4 + x_4^3 x_5 - x_4^2 x_5^2 + x_4 x_5^3 + x_2 x_5^2 x_6 - x_4^2 x_6^2 + x_5 x_6^3 - x_4 x_5^2 x_6^2 + x_5^2 x_6^2 + x_5^3 x_6^2, \\
& x_3 x_4^2 - x_4^4 - x_4^3 x_5^2 - x_4^2 x_5^3 - x_4 x_6^2 + x_5 x_6^3 - x_4 x_5^2 x_6^2 + x_5^2 x_6^2 + x_5^3 x_6^2, \\
& x_4^2 x_5^2 - x_4^3 x_5^2 + x_4^2 x_6^2 + x_5 x_6^3 - x_4 x_5^2 x_6^2 + x_5^2 x_6^2 + x_5^3 x_6^2, \\
& x_3^3 x_5 + x_4^3 x_5^2 - x_4^2 x_5^3 + x_3 x_4 x_6 - x_4^3 x_6^2 + x_4^2 x_5^2 x_6 + x_5 x_6^3 - x_4 x_5^2 x_6^2 + x_5^2 x_6^2 + x_5^3 x_6^2, \\
& -x_4^4 + x_4^3 x_5 + x_3 x_5^2 - x_4^2 x_5^3 + x_4^2 x_6^2 + x_5 x_6^3 - x_4 x_5^2 x_6^2 + x_5^2 x_6^2 + x_5^3 x_6^2, \\
& -x_4^4 + x_4^3 x_5 + x_5^4 + x_4^3 x_6 + x_4^2 x_5^2 x_6 + x_5 x_6^3 - x_4 x_5^2 x_6^2 + x_5^2 x_6^2 + x_5^3 x_6^2, \\
& x_4^4 - x_4^3 x_5 + x_4 x_5^3 - x_5^4 + x_3 x_5^2 x_6 - x_4^2 x_6^2 + x_5 x_6^3 - x_4 x_5^2 x_6^2 + x_5^2 x_6^2 - x_5^3 x_6^2, \\
& x_4^4 - x_4^3 x_5 + x_4 x_5^3 - x_5^4 + x_3 x_5^2 x_6 - x_4^2 x_6^2 + x_5 x_6^3 - x_4 x_5^2 x_6^2 + x_5^2 x_6^2 - x_5^3 x_6^2 \} ; *)
\end{aligned}$$

```
Length[G]
```

```
46
```

```
isEfficient[G, LM, bdry, varList]
```

```
True
```

```
isThetaEfficient[G, LM, TM, bdry, varList, verbose = True]
```

```
Condition 1 of Proposition 3.1 is True.
```

```
(numProds = 276) >= (numQ = 177)
```

```
The map  $\vartheta$  is surjective.
```

```
True
```

```
borBasis = makeBorderBasisOfI[G, bdry, LM];
```

## Find the tangent space relations and the dimension of the tangent space at $[I]$ :

In this case, we don't use the "usual" command **tanSpaceDim** (after finding the tangent space relations) since we want to work modulo a large prime to conserve memory.

```
{aLst, allTanSpaceRelns} = makeTanSpaceRelns[borBasis, OO, bdry, varList];
```

```
PrimeQ[32 713]
```

```
True
```

```
MatrixRank[allTanSpaceRelns, Modulus  $\rightarrow$  32 713]
```

```
6821
```

As noted in Section 8.4 of the paper, this is exactly the right value to give us genericity. The dimension of  $F(U)$  in this case is

$\lambda \cdot \tau + 6 + 3 \cdot 3 = 46 \cdot 15 + 6 + 9 = 705$ . So  $[I]$  lies on an elementary component of dimension 705.

```
7526 - 6821
```

```
705
```
