# Supplementary material for: Some elementary components of the Hilbert scheme of points
Source: arXiv:1407.1440 ancillary file (2016-01-21)
Supplement: Supplementary file 7 [file case__1_6_6_10_0_.pdf]

# Case (1,6,6,10,0).

This file accompanies the paper *Some Elementary Components of the Hilbert Scheme of Points*, to appear in the *Rocky Mountain Journal of Mathematics*.

Author: Mark Huibregtse

Affiliation: Skidmore College .

Email address: mhuibreg@skidmore.edu .

This notebook contains the details of the example presented in Section 8.3 of the paper.

Assign the number of variables  $n$ , the list of variables  $\{x_1, \dots, x_n\}$ , and the list of null substitutions  $\{x_1 \rightarrow 0, \dots, x_n \rightarrow 0\}$ .

```
n = 6;  
varList = Table[xi, {i, 1, n}];  
nullSubs = makeNullSubLst[varList];
```

Make the lex-segment complement order ideal for Hilbert function (1,6,6,10,0), and the set of boundary monomials.

```
OO = makeOrderIdeal[{1, 6, 6, 10}, varList]  
{1, x1, x2, x3, x4, x5, x6, x42, x4 x5, x4 x6, x52, x5 x6,  
x62, x43, x42 x5, x42 x6, x4 x52, x4 x5 x6, x4 x62, x53, x52 x6, x5 x62, x63}  
  
μ = Length[OO]  
23  
  
bdry = bdryMonoms[OO, varList]  
{x12, x1 x2, x1 x3, x1 x4, x1 x5, x1 x6, x22, x2 x3, x2 x4, x2 x5, x2 x6, x32, x3 x4, x3 x5,  
x3 x6, x4 x42, x4 x4 x5, x4 x4 x6, x4 x52, x4 x5 x6, x4 x62, x5 x42, x5 x4 x5, x5 x4 x6, x5 x52,  
x5 x5 x6, x5 x62, x6 x42, x6 x4 x5, x6 x4 x6, x6 x52,  
x6 x5 x6, x6 x62, x3 x42, x3 x4 x5, x3 x4 x6, x3 x52, x3 x5 x6, x3 x62, x4 x43, x4 x42 x5, x4 x42 x6,  
x4 x4 x52, x4 x4 x5 x6, x4 x4 x62, x4 x53, x4 x52 x6, x4 x5 x62, x4 x63, x5 x43, x5 x42 x5, x5 x42 x6,  
x5 x4 x52, x5 x4 x5 x6, x5 x4 x62, x5 x53, x5 x52 x6, x5 x5 x62, x5 x63, x6 x44, x6 x43 x5, x6 x43 x6,  
x6 x42 x52, x6 x42 x5 x6, x6 x42 x62, x6 x54, x6 x53 x6, x6 x52 x62, x6 x64}
```

```
numBdry = Length[bdry]
```

78

Form the sets of leading and trailing monomials LM and TM.

```
mins = minBdryMons[OO, bdry, varList]
```

$$\{x_1^2, x_1 x_2, x_1 x_3, x_1 x_4, x_1 x_5, x_1 x_6, x_2^2, x_2 x_3, x_2 x_4, x_2 x_5, x_2 x_6, x_3^2, x_3 x_4, x_3 x_5, x_3 x_6, x_4^2, x_4^3 x_5, x_4^3 x_6, x_4^2 x_5^2, x_4^2 x_5 x_6, x_4^2 x_6^2, x_4 x_5^3, x_4 x_5^2 x_6, x_4 x_5 x_6^2, x_4 x_6^3, x_5^4, x_5^3 x_6, x_5^2 x_6^2, x_5 x_6^3, x_6^4\}$$

```
LM = Take[mins, 15]
```

$$\{x_1^2, x_1 x_2, x_1 x_3, x_1 x_4, x_1 x_5, x_1 x_6, x_2^2, x_2 x_3, x_2 x_4, x_2 x_5, x_2 x_6, x_3^2, x_3 x_4, x_3 x_5, x_3 x_6\}$$

```
 $\lambda$  = Length[LM]
```

```
15
```

```
maxes = maxBasisMons[OO, bdry, varList]
```

$$\{x_1, x_2, x_3, x_4^3, x_4^2 x_5, x_4^2 x_6, x_4 x_5^2, x_4 x_5 x_6, x_4 x_6^2, x_5^3, x_5^2 x_6, x_5 x_6^2, x_6^3\}$$

```
TM = Take[maxes, -10]
```

$$\{x_4^3, x_4^2 x_5, x_4^2 x_6, x_4 x_5^2, x_4 x_5 x_6, x_4 x_6^2, x_5^3, x_5^2 x_6, x_5 x_6^2, x_6^3\}$$

```
 $\tau$  = Length[TM]
```

```
10
```

Randomly generate a short list of polynomials  $G$ , test for efficiency and  $\theta$ -efficiency, and make the associated border basis of the distinguished ideal associated to the short list.

To generate a new random example, execute the immediately-following cell. To re-run a previously-executed example that works (i.e., produces a generic ideal), un-comment the assignment cell that follows the next.

```
G = makeShortListOfIdealGenerators[LM, TM]
```

$$\begin{aligned} &\{x_1^2 - x_4^3 - x_4^2 x_5 + x_4 x_5^2 - x_5^3 - x_4^2 x_6 - x_4 x_5 x_6 - x_5^2 x_6 + x_5 x_6^2, \\ &x_1 x_2 - x_4^3 + x_4^2 x_5 - x_4 x_5^2 + x_5^3 + x_4 x_5 x_6 - x_4 x_6^2 - x_5 x_6^2 + x_6^3, \\ &x_1 x_3 - x_4^2 x_5 + x_4^2 x_6 + x_4 x_5 x_6 + x_5^2 x_6 - x_4 x_6^2 - x_6^3, \\ &x_1 x_4 + x_4^3 + x_4^2 x_5 + x_4 x_5^2 - x_5^3 + x_4 x_5 x_6 - x_5^2 x_6 + x_4 x_6^2 - x_6^3, \\ &x_1 x_5 - x_4^2 x_5 + x_4^2 x_6 - x_4 x_5 x_6 + x_5^2 x_6 - x_4 x_6^2 - x_5 x_6^2 + x_6^3, \\ &-x_4^3 + x_4^2 x_5 - x_4 x_5^2 - x_5^3 + x_1 x_6 + x_4^2 x_6 + x_4 x_5 x_6 - x_5^2 x_6 + x_4 x_6^2 - x_5 x_6^2 + x_6^3, \\ &x_2^2 - x_4^3 + x_4^2 x_5 - x_4^2 x_6 - x_4 x_5 x_6 + x_5^2 x_6 - x_4 x_6^2 + x_5 x_6^2 - x_6^3, \\ &x_2 x_3 - x_4^3 + x_4 x_5^2 - x_4 x_5 x_6 + x_5^2 x_6 - x_5 x_6^2, x_2 x_4 + x_4^3 + x_4^2 x_5 + x_4^2 x_6 + x_4 x_5 x_6 + x_4 x_6^2 + x_5 x_6^2 - x_6^3, \\ &-x_4^3 + x_2 x_5 + x_4^2 x_5 - x_5^3 - x_4 x_5 x_6 + x_4 x_6^2 + x_5 x_6^2, x_4^2 x_5 - x_4 x_5^2 - x_5^3 + x_2 x_6 + x_4^2 x_6 - x_4 x_6^2 + x_5 x_6^2 + x_6^3, \\ &x_5^2 - x_4^3 + x_4^2 x_5 - x_4 x_5^2 + x_5^3 + x_4^2 x_6 + x_4 x_6^2 - x_5 x_6^2, x_3 x_4 + x_4^2 x_5 - x_5^3 + x_4^2 x_6 - x_4 x_5 x_6 + x_5^2 x_6, \\ &x_3 x_5 + x_4 x_5^2 - x_5^3 - x_4^2 x_6 + x_4 x_5 x_6 + x_4 x_6^2 + x_5 x_6^2 - x_6^3, \\ &x_4 x_5^2 + x_3 x_6 + x_4^2 x_6 - x_4 x_5 x_6 - x_4 x_6^2 + x_5 x_6^2 - x_6^3\} \end{aligned}$$

The following cell contains an example that works. To use it, just un-comment the cell and shift-enter it, then continue executing the remaining cells in the notebook.

```
( * G = { x1^2 - x4^3 - x4^2 x5 + x4 x5^2 - x5^3 - x4^2 x6 - x4 x5 x6 - x5^2 x6 + x5 x6^2,
  x1 x2 - x4^3 + x4^2 x5 - x4 x5^2 + x5^3 + x4 x5 x6 - x4 x6^2 - x5 x6^2 + x6^3,
  x1 x3 - x4^2 x5 + x4^2 x6 + x4 x5 x6 + x5^2 x6 - x4 x6^2 - x6^3, x1 x4 + x4^3 + x4^2 x5 + x4 x5^2 - x5^3 +
  x4 x5 x6 - x5^2 x6 + x4 x6^2 - x6^3, x1 x5 - x4^2 x5 + x4^2 x6 - x4 x5 x6 + x5^2 x6 - x4 x6^2 - x5 x6^2 + x6^3,
  -x4^3 + x4^2 x5 - x4 x5^2 - x5^3 + x1 x6 + x4^2 x6 + x4 x5 x6 - x5^2 x6 + x4 x6^2 - x5 x6^2 + x6^3,
  x2^2 - x4^3 + x4^2 x5 - x4^2 x6 - x4 x5 x6 + x5^2 x6 - x4 x6^2 + x5 x6^2 - x6^3, x2 x3 - x4^3 + x4 x5^2 - x4 x5 x6 + x5^2 x6 - x5 x6^2,
  x2 x4 + x4^3 + x4^2 x5 + x4^2 x6 + x4 x5 x6 + x5^2 x6 - x6^3, -x4^3 + x2 x5 + x4^2 x5 - x5^3 - x4 x5 x6 + x4 x6^2 + x5 x6^2,
  x4^2 x5 - x4 x5^2 - x5^3 + x2 x6 + x4^2 x6 - x4 x6^2 + x5 x6^2 + x6^3, x3^2 - x4^3 + x4^2 x5 - x4 x5^2 + x5^3 + x4^2 x6 + x4 x6^2 - x5 x6^2,
  x3 x4 + x4^2 x5 - x5^3 + x4^2 x6 - x4 x5 x6 + x5^2 x6, x3 x5 + x4 x5^2 - x5^3 - x4^2 x6 + x4 x5 x6 + x4 x6^2 + x5 x6^2 - x6^3,
  x4 x5^2 + x3 x6 + x4^2 x6 - x4 x5 x6 - x4 x6^2 + x5 x6^2 - x6^3 } * )
```

**Length[G]**

15

**isEfficient[G, LM, bdry, varList]**

True

**isThetaEfficient[G, LM, TM, bdry, varList, verbose = True]**

Condition 1 of Proposition 3.1 is True.

(numProds = 90) < (numQ = 91)

The map  $\vartheta$  is not surjective.

False

```
borBasis = makeBorderBasisOfI[G, bdry, LM]
```

```
{ x1^2 - x4^3 - x4^2 x5 + x4 x5^2 - x5^3 - x4^2 x6 - x4 x5 x6 - x5^2 x6 + x5 x6^2,
  x1 x2 - x4^3 + x4^2 x5 - x4 x5^2 + x5^3 + x4 x5 x6 - x4 x6^2 - x5 x6^2 + x6^3,
  x1 x3 - x4^2 x5 + x4^2 x6 + x4 x5 x6 + x5^2 x6 - x4 x6^2 - x6^3,
  x1 x4 + x4^3 + x4^2 x5 + x4 x5^2 - x5^3 + x4 x5 x6 - x5^2 x6 + x4 x6^2 - x6^3,
  x1 x5 - x4^2 x5 + x4^2 x6 - x4 x5 x6 + x5^2 x6 - x4 x6^2 - x5 x6^2 + x6^3,
  -x4^3 + x4^2 x5 - x4 x5^2 - x5^3 + x1 x6 + x4^2 x6 + x4 x5 x6 - x5^2 x6 + x4 x6^2 - x5 x6^2 + x6^3,
  x2^2 - x4^3 + x4^2 x5 - x4^2 x6 - x4 x5 x6 + x5^2 x6 - x4 x6^2 + x5 x6^2 - x6^3,
  x2 x3 - x4^3 + x4 x5^2 - x4 x5 x6 + x5^2 x6 - x5 x6^2, x2 x4 + x4^3 + x4^2 x5 + x4^2 x6 + x4 x5 x6 + x4 x6^2 + x5 x6^2 - x6^3,
  -x4^3 + x2 x5 + x4^2 x5 - x5^3 - x4 x5 x6 + x4 x6^2 + x5 x6^2, x4^2 x5 - x4 x5^2 - x5^3 + x2 x6 + x4^2 x6 - x4 x6^2 + x5 x6^2 + x6^3,
  x5^3 - x4^3 + x4^2 x5 - x4 x5^2 + x5^3 + x4^2 x6 + x4 x6^2 - x5 x6^2, x3 x4 + x4^2 x5 - x5^3 + x4^2 x6 - x4 x5 x6 + x5^2 x6,
  x3 x5 + x4 x5^2 - x5^3 - x4^2 x6 + x4 x5 x6 + x4 x6^2 + x5 x6^2 - x6^3,
  x4 x5^2 + x3 x6 + x4^2 x6 - x4 x5 x6 - x4 x6^2 + x5 x6^2 - x6^3, x1 x4^2, x1 x4 x5, x1 x4 x6, x1 x5^2,
  x1 x5 x6, x1 x6^2, x2 x4^2, x2 x4 x5, x2 x4 x6, x2 x5^2, x2 x5 x6, x2 x6^2, x3 x4^2, x3 x4 x5,
  x3 x4 x6, x3 x5^2, x3 x5 x6, x3 x6^2, x1 x4^3, x1 x4^2 x5, x1 x4^2 x6, x1 x4 x5^2, x1 x4 x5 x6,
  x1 x4 x6^2, x1 x5^3, x1 x5^2 x6, x1 x5 x6^2, x1 x6^3, x2 x4^3, x2 x4^2 x5, x2 x4^2 x6, x2 x4 x5^2,
  x2 x4 x5 x6, x2 x4 x6^2, x2 x5^3, x2 x5^2 x6, x2 x5 x6^2, x2 x6^3, x3 x4^3, x3 x4^2 x5, x3 x4^2 x6,
  x3 x4 x5^2, x3 x4 x5 x6, x3 x4 x6^2, x3 x5^3, x3 x5^2 x6, x3 x5 x6^2, x3 x6^3, x4^4, x4^3 x5, x4^3 x6,
  x4^2 x5^2, x4^2 x5 x6, x4^2 x6^2, x4 x5^3, x4 x5^2 x6, x4 x5 x6^2, x4 x6^3, x5^4, x5^3 x6, x5^2 x6^2, x5 x6^3, x6^4 }
```

Find the tangent space relations and the dimension of the tangent space at [I]:

```
{aLst, allTanSpaceRelns} = makeTanSpaceRelns[borBasis, OO, bdry, varList];
```

```
tanSpaceDim[Length[aLst], allTanSpaceRelns]
```

```
165
```

As shown in Section 8.3 of the paper, a tangent space dimension of 165 implies that the ideal  $I = (G) = (\text{borBasis})$  is generic.
