# Supplementary material for: Some elementary components of the Hilbert scheme of points
Source: arXiv:1407.1440 ancillary file (2016-01-21)
Supplement: Supplementary file 8 [file plausible_shapes.pdf]

# Plausible Shapes

This file accompanies the paper *Some Elementary Components of the Hilbert Scheme of Points*, to appear in the *Rocky Mountain Journal of Mathematics*.

Author: Mark Huibregtse

Affiliation: Skidmore College .

Email address: mhuibreg@skidmore.edu .

This notebook contains the computations justifying the plausible shapes reported in equation (1) of the introduction to the paper, as well as the non-example reported in the last paragraph of section 10.3. We use the function `genericityIsPlausible`, which is coded in the last portion of the notebook of utility functions.

---

## $(n, 2, 2, 3)$ is plausible for $5 \leq n \leq 50\,000$ (at least)

```
genericityIsPlausible[4, 2, 2, 3]
```

```
False
```

```
DeleteDuplicates[Table[genericityIsPlausible[n, 2, 2, 3], {n, 5, 50 000}]]
```

```
{True}
```

---

## $(n, 2, 2, 4)$ is plausible for $5 \leq n \leq 50\,000$ (at least)

```
genericityIsPlausible[4, 2, 2, 4]
```

```
False
```

```
DeleteDuplicates[Table[genericityIsPlausible[n, 2, 2, 4], {n, 5, 50 000}]]
```

```
{True}
```

---

## $(n, 3, 3, 4)$ is plausible for $5 \leq n \leq 17$

```
genericityIsPlausible[4, 3, 3, 4]
```

```
False
```

```
genericityIsPlausible[4, 3, 3, 18]
```

```
False
```

```
DeleteDuplicates[Table[genericityIsPlausible[n, 3, 3, 4], {n, 5, 17}]]
{True}
```

---

## $(n, 3, 3, 5)$ is plausible for $5 \leq n \leq 25$

```
genericityIsPlausible[4, 3, 3, 5]
False

genericityIsPlausible[4, 3, 3, 26]
False

DeleteDuplicates[Table[genericityIsPlausible[n, 3, 3, 5], {n, 5, 25}]]
{True}
```

---

## $(n, 4, 2, 6)$ is plausible for $16 \leq n \leq 50\,000$ (at least)

```
genericityIsPlausible[15, 4, 2, 6]
False

DeleteDuplicates[Table[genericityIsPlausible[n, 4, 2, 6], {n, 16, 50\,000}]]
{True}
```

---

## $(n, 4, 3, 6)$ is plausible for $8 \leq n \leq 120$

```
genericityIsPlausible[7, 4, 3, 6]
False

genericityIsPlausible[121, 4, 3, 6]
False

DeleteDuplicates[Table[genericityIsPlausible[n, 4, 3, 6], {n, 8, 120}]]
{True}
```

---

## $(50, \kappa, 4, 6)$ is plausible for $7 \leq k \leq 22$

```
genericityIsPlausible[50, 6, 4, 6]
False
```

```
genericityIsPlausible[50, 23, 4, 6]
False

DeleteDuplicates[Table[genericityIsPlausible[50,  $\kappa$ , 4, 6], { $\kappa$ , 7, 22}]]
{True}
```

## $(50, \kappa, 4, 8)$ is plausible for $6 \leq \kappa \leq 14$

```
genericityIsPlausible[50, 5, 4, 8]
False

genericityIsPlausible[50, 15, 4, 8]
False

DeleteDuplicates[Table[genericityIsPlausible[50,  $\kappa$ , 4, 8], { $\kappa$ , 6, 14}]]
{True}
```

## $(n, 3, 10, 11)$ is NOT plausible for $4 \leq n \leq 50\,000$ (at least)

```
DeleteDuplicates[Table[genericityIsPlausible[n, 3, 10, 11], {n, 4, 50 000}]]
{False}
```

The reason for this failure is that there are too few tangent space relations. As shown in section 10.3, the size of  $A_s$ , the set of indeterminates  $a_{\{i,j\}}$  that can appear in the tangent space relations of degree  $s$ , grows with dominant term  $O(n^{2r-1}) = O(n^{19})$ , whereas the number of tangent space relations of degree  $s$  grows with dominant term  $O(n^{r+1}) = O(n^{11})$ .

```
DeleteDuplicates[Table[hasEnoughReIns[n, 3, 10, 11], {n, 5, 50 000}]]
{False}

DeleteDuplicates[Table[thetaEfficiencyIsLikely[n, 3, 10, 11], {n, 5, 50 000}]]
{True}
```

On the other hand, there are plausible shapes with  $r = 10$ ,  $s = 11$ :

```
Clear[resultIsTrue]

resultIsTrue[threeTuple_] := threeTuple[[3]] == True;

Select[Flatten[Table[{n,  $\kappa$ , genericityIsPlausible[n,  $\kappa$ , 10, 11]},
  {n, 45, 65}, { $\kappa$ , 10, 40}], 1], resultIsTrue]

{{45, 22, True}, {45, 23, True}, {45, 24, True}, {45, 25, True}, {45, 26, True},
 {45, 27, True}, {45, 28, True}, {45, 29, True}, {45, 30, True}, {45, 31, True},
```

[illegible]

```

{58, 38, True}, {58, 39, True}, {58, 40, True}, {59, 27, True}, {59, 28, True},
{59, 29, True}, {59, 30, True}, {59, 31, True}, {59, 32, True}, {59, 33, True},
{59, 34, True}, {59, 35, True}, {59, 36, True}, {59, 37, True}, {59, 38, True},
{59, 39, True}, {59, 40, True}, {60, 28, True}, {60, 29, True}, {60, 30, True},
{60, 31, True}, {60, 32, True}, {60, 33, True}, {60, 34, True}, {60, 35, True},
{60, 36, True}, {60, 37, True}, {60, 38, True}, {60, 39, True}, {60, 40, True},
{61, 28, True}, {61, 29, True}, {61, 30, True}, {61, 31, True}, {61, 32, True},
{61, 33, True}, {61, 34, True}, {61, 35, True}, {61, 36, True}, {61, 37, True},
{61, 38, True}, {61, 39, True}, {61, 40, True}, {62, 29, True}, {62, 30, True},
{62, 31, True}, {62, 32, True}, {62, 33, True}, {62, 34, True}, {62, 35, True},
{62, 36, True}, {62, 37, True}, {62, 38, True}, {62, 39, True}, {62, 40, True},
{63, 29, True}, {63, 30, True}, {63, 31, True}, {63, 32, True}, {63, 33, True},
{63, 34, True}, {63, 35, True}, {63, 36, True}, {63, 37, True}, {63, 38, True},
{63, 39, True}, {63, 40, True}, {64, 29, True}, {64, 30, True}, {64, 31, True},
{64, 32, True}, {64, 33, True}, {64, 34, True}, {64, 35, True}, {64, 36, True},
{64, 37, True}, {64, 38, True}, {64, 39, True}, {64, 40, True}, {65, 30, True},
{65, 31, True}, {65, 32, True}, {65, 33, True}, {65, 34, True}, {65, 35, True},
{65, 36, True}, {65, 37, True}, {65, 38, True}, {65, 39, True}, {65, 40, True}

```
