# Supplementary material for: Some elementary components of the Hilbert scheme of points
Source: arXiv:1407.1440 ancillary file (2016-01-21)
Supplement: Supplementary file 9 [file utility_functions.pdf]

# Utility Functions

This file accompanies the paper *Some Elementary Components of the Hilbert Scheme of Points*, to appear in the *Rocky Mountain Journal of Mathematics*.

Author: Mark Huibregtse

Affiliation: Skidmore College .

Email address: mhuibreg@skidmore.edu .

This notebook collects together a variety of functions for working with border bases and border basis schemes. Throughout, we often refer to an order ideal as a “basis set” or “basis.” This notebook should be evaluated before any of the other notebooks that use the functions provided here are evaluated.

This can be done using the **Evaluate Notebook** option under the **Evaluation** menu.

---

## I. Basic utility functions

Assign the number of variables and construct a list of the variables  $x_i$  and a list of “null substitutions”  $x_i \rightarrow 0$ .

```
n = 3;
varList = Table[xi, {i, 1, n}]

{x1, x2, x3}

makeNullSubLst[itemList_] := Table[itemList[[i]] → 0, {i, 1, Length[itemList]};
nullSubs = makeNullSubLst[varList]

{x1 → 0, x2 → 0, x3 → 0}
```

The following function returns a list of the monomials of the given degree  $\text{deg}$  in the variables  $x_{\text{minVar}} \dots x_{\text{maxVar}}$ . The list is in decreasing lex order ( $x_1 > x_2 > \dots > x_n$ ).

```
allDegNMonoms[deg_, maxVar_, minVar_] := Module[{result, i},
  (
    If[deg == 0,
      (
        result = {1}
      ),
      (
        If[minVar == maxVar,
          (
            result = {xminVardeg};
          ),
          (
            result = Flatten[
              Table[xminVardeg-i * allDegNMonoms[i, maxVar, minVar + 1], {i, 0, deg}], 1];
          )];
      )];
  result
];
```

Example:

```
allDegNMonoms[5, 3, 1]
```

```
{x15, x14 x2, x14 x3, x13 x22, x13 x2 x3, x13 x32, x12 x23, x12 x22 x3, x12 x2 x32, x12 x33,
  x1 x24, x1 x23 x3, x1 x22 x32, x1 x2 x33, x1 x34, x25, x24 x3, x23 x32, x22 x33, x2 x34, x35}
```

The next function sorts a list of monomials in  $x_1, \dots, x_n$  into decreasing lex order, degree by degree.

This function makes use of the fact that the built-in *Mathematica* function **MonomialList** returns the list of monomials using a monomial order that can be specified. The function first adds the monomials in the list together and then applies **MonomialList** to this sum. We use the monomial order option **NegativeDegreeLexicographic** to generate the list in decreasing lex order, degree-by-degree, with the degrees increasing. If the input set of monomials is empty, the set {0} is returned.

```
sortInLexOrder[monLst_, varLst_] :=
  MonomialList[Apply[Plus, monLst], varLst, NegativeDegreeLexicographic];

sortInLexOrder[{x1, x22 x4, x3 x5, x43, x1 x52}, {x1, x2, x3, x4, x5}]
{x1, x3 x5, x1 x52, x22 x4, x43}
```

```
sortInLexOrder[{}, {x1, x2, x3, x4, x5}]
{0}
```

The next function `coeffOfTerm` extracts the (scalar) coefficient of a given monomial in a given polynomial.

Here is an example of *Mathematica*'s built-in **Coefficient** function in action:

```
Coefficient[x1 - x23 - (x13 - 7)^2 + 8 x3 + 3 x1 x3 - 2 x2 x32, x3]
8 + 3 x1
```

In the sequel, we want to be able to extract the coefficient of the desired monomial (in the example,  $x_3$ ) only, and not have the “variable coefficients” such as  $3 x_1$  included. To achieve this behavior, we can use the following function that returns the output of **Coefficient** after substituting 0 into each of the variables; it also handles the special case of the monomial 1.

```
coeffOfTerm[poly_, mon_, varList_] := Module[{result, nullSubs},
(
  nullSubs = makeNullSubLst[varList] ;
  If[(mon /. nullSubs) == 0,
    result = Coefficient[poly, mon] /. nullSubs, result = poly /. nullSubs];
  result
)]
```

Examples:

```
varList
```

```
{x1, x2, x3}
```

```
coeffOfTerm[x1 - x23 - (x13 - 7)^2 + 8 x3 + 3 x1 x3 - 2 x2 x32, x3, varList]
8
```

```
coeffOfTerm[x1 - x23 - (x13 - 7)^2 + 8 x3 + 3 x1 x3 - 2 x2 x32, 1, varList]
-49
```

The following function takes a polynomial “poly” (in  $x_1 \dots x_n$ ) and a list of monomials “targetMonomLst,” and constructs the list of coefficients that each of the target monomials has in poly.

```
makeCoeffLst[poly_, targetMonomLst_, varList_] := Table[
  coeffOfTerm[poly, targetMonomLst[[i]], varList], {i, 1, Length[targetMonomLst]}];
```

The next function generalizes the preceding. It accepts a list of polynomials

"polyLst" and the targetMonomLst, and constructs the list of the coefficient lists corresponding to the polynomials in polyLst.

```
makeListOfCoeffLsts[polyLst_, targetMonomLst_, varList_] := Table[
  makeCoeffLst[polyLst[[i]], targetMonomLst, varList], {i, 1, Length[polyLst]}];
```

The next function returns the index in the given list where the given item occurs (assuming the item appears once in the list).

```
indexOf[item_, lst_] := Position[lst, item][[1]][[1]];

indexOf[4, Table[i^2, {i, 1, 5}]]
2
```

The next function returns True if monomial m1 divides monomial m2, and False otherwise.

```
monomDivides[m1_, m2_, varList_] :=
Module[{exponentList1, exponentList2, result, okSoFar, i, numVars},
(
  numVars = Length[varList];
  exponentList1 = Table[Exponent[m1, varList[[i]]], {i, 1, numVars}];
  exponentList2 = Table[Exponent[m2, varList[[i]]], {i, 1, numVars}];
  okSoFar = True;
  i = 1;
  While[okSoFar && (i ≤ numVars),
    (
      okSoFar = exponentList1[[i]] ≤ exponentList2[[i]];
      i = i + 1;
    )];
  result = okSoFar;
  result
)];
```

```
monomDivides[x2 x3, x13 x2 x32, {x1, x2, x3}]
```

```
True
```

```
monomDivides[x13, x12, {x1, x2}]
```

```
False
```

## II. Utilities for General Border Bases and Border Pre-Bases

The next function constructs the set of boundary monomials associated to a given order ideal (entered as a list of monomials called “basis”) in the variables of `varList`.

```
bdryMonoms[basis_, varList_] :=
Module[{result, i, j, numBasis, curMon, curMonInBasis, n},
(
  n = Length[varList];
  numBasis = Length[basis];
  result = {};

  For[i = 1, i ≤ n, i++,
  (
    For[j = 1, j ≤ numBasis, j++,
    (
      curMon = varList[[i]] * basis[[j]];
      curMonInBasis = MemberQ[basis, curMon];
      If[! curMonInBasis, result = Append[result, curMon]];
    )];
  )];
  result = sortInLexOrder[DeleteDuplicates[result], varList]
)];
```

Example:

```
bdry = bdryMonoms[{1, x1, x2, x3, x2 x3, x32, x33}, {x1, x2, x3}]
{x12, x1 x2, x1 x3, x22, x1 x2 x3, x1 x32, x22 x3, x2 x32, x1 x33, x2 x33, x34}
```

The following function takes a polynomial that is a linear combination of basis and boundary monomials (typical case: an S-polynomial of two members of a border basis or pre-basis), and reduces the polynomial modulo the border basis/pre-basis. The result is a linear combination of basis monomials only.

The following code depends for its correctness on having the border basis list (“`borBasis`”) in the same order as the list of boundary monomials (“`bdry`”). The first input “poly” is a polynomial that is a linear combination of basis and boundary monomials. The output is the polynomial reduced modulo the border basis (which is accordingly a linear combination of basis monomials only). This is

not a fully general reduction procedure, but it is all we need for computing linear syzygies and the tangent space relations associated to a basis of linear syzygies.

```
reducePoly[poly_, bdry_, borBasis_, varList_] :=
Module[{result, curCoeff, numBdry, i},
(
  result = poly;
  numBdry = Length[bdry];

  For[i = 1, i ≤ numBdry, i++,
    (
      curCoeff = coeffOfTerm[result, bdry[[i]], varList];
      result = result - curCoeff * borBasis[[i]];
    )];
  result
)];
```

The next function constructs a basis of the linear syzygies of the given border Basis. It implements the algorithm described in Section 2.3 of the paper “Some Elementary Components of the Hilbert Scheme of Points.”

```
makeLinearSyzygies[bdry_, borBasis_, varList_] :=
Module[{numBdry, result, i, j, p, z, T, numTargets, multipliers, numMultipliers,
  products, numProducts, theMatrix, nulSp, curMonSyz, curCoeff, numVars},
(
  numVars = Length[varList];
  numBdry = Length[bdry];

  (* We next form the set T
    of "target monomials" as described in Section 2.3 *)
  T = DeleteDuplicates[Join[bdry, Flatten[
    Table[varList[[i]] * bdry[[j]], {i, 1, numVars}, {j, 1, numBdry}]]]];
  numTargets = Length[T];

  (* The set "products" is the set of
    images of the basis elements  $e_{\alpha,j}$  of the vector space E *)
  multipliers = Join[{1}, varList];
  numMultipliers = numVars + 1;
  products = Flatten[Table[multipliers[[i]] * borBasis[[j]],
    {i, 1, numMultipliers}, {j, 1, numBdry}]];
  numProducts = numBdry * numMultipliers;
```

```

(* "theMatrix is the matrix of
   the map  $\sigma$  with respect to the bases  $\{e_{\{\alpha,j\}}\}$  and T *)
theMatrix = Transpose[makeListOfCoeffLsts[products, T, varList]];
(* This matrix must have maximal rank = numTargets,
   since the map  $\sigma$  is surjective *)

nulSp = NullSpace[theMatrix]; (* This is a list of length
   (numProducts - numTargets) consisting of lists of length numProducts *)

(* Now we must assemble the
   syzygies corresponding to each of the lists in nulSp *)
(* This list "result" is the output of the function. *)

result = {};
For[p = 1, p ≤ numProducts - numTargets, p++,
  ((* Extract the pth monomial syzygy *))
  curMonSyz = Table[0, {i, 1, numBdry}];
  For[z = 1, z ≤ numProducts, z++,
    (
      curCoeff = nulSp[[p]][[z]];
      i = Quotient[z - 1, numBdry] + 1;
      j = Mod[z - 1, numBdry] + 1;
      curMonSyz[[j]] = curMonSyz[[j]] + curCoeff * multipliers[[i]];
    )];
  result = Append[result, curMonSyz];
];

result
];

```

The next function constructs the generators of the ideal of the border basis scheme (denoted  $\phi_i^{j,j'}$  in Section 2.4 of the paper). This is done by computing the reduced S-polynomials  $\bar{S}(G_j, G_{j'})$  relative to the “generic O-border pre-basis”  $\{G_j\}$  and extracting the coefficients of each of the basis monomials.

```

makeBorBasisSchemeIdealGenerators[basisSet_, varList_] :=
Module[{result, i, j, bdry, numBdry, numBasis,
  genericBorderPreBasis, linearMonomialSyz, genericLinearSyzLst,
  bdrySyzAppliedToGenericPreBasis, lstOfReducedSPolys, numSyz},
(
  bdry = bdryMonoms[basisSet, varList];
  numBdry = Length[bdry];
  numBasis = Length[basisSet];
  genericBorderPreBasis =
    Table[bdry[[j]] -  $\sum_{i=1}^{\text{numBasis}} C_{\{i,j\}}$  basisSet[[i]], {j, 1, numBdry}];
  (* We now find a basis of the linear syzygies of the boundary monomials *)
  linearMonomialSyz = makeLinearSyzygies[bdry, bdry, varList];

  numSyz = Length[linearMonomialSyz];

  (* Construct list of generic linear
    syzygies from the syzygies of the boundary monomials *)

  genericLinearSyzLst = {};
  For[i = 1, i ≤ numSyz, i++,
    (
      bdrySyzAppliedToGenericPreBasis =
        genericBorderPreBasis.linearMonomialSyz[[i]];
      genericLinearSyzLst = Append[genericLinearSyzLst, linearMonomialSyz[[i]] -
        makeCoeffLst[bdrySyzAppliedToGenericPreBasis, bdry, varList]];
    )];

  lstOfReducedSPolys =
    Table[genericLinearSyzLst[[i]].genericBorderPreBasis, {i, 1, numSyz}];
  result = Flatten[makeListOfCoeffLsts[lstOfReducedSPolys, basisSet, varList]];
  result
)];

```

The next function generates a list of the indeterminates  $C_{\{i,j\}}$  that are the coefficients in the generic O-border pre-basis.

```

makeCLst[numBasis_, numBdry_] :=
  Flatten[Table[C{i,j}, {j, 1, numBdry}, {i, 1, numBasis}]]

```



The next function takes a given border (pre)basis, and constructs the list of substitutions  $\{C_{\{i,j\}} \rightarrow c_{\{i,j\}}\}$  that correspond to it. It is assumed that the border (pre)basis list is in the same order as the list of boundary monomials.

```
makeCCoordsOfBorBasis[borBasis_, basisSet_, bdry_, varList_] :=
Module[{numBasis, numBdry, result, listOfCs, i, j},
(
numBasis = Length[basisSet];
numBdry = Length[bdry];
result = {};

For[j = 1, j ≤ numBdry, j++,
(
For[i = 1, i ≤ numBasis, i++,
(
result = Append[result,
C{i,j} → -coeffOfTerm[borBasis[[j]], basisSet[[i]], varList] ];
)]];
result
)];
```

The next function reverses the previous one: it takes a list of substitutions  $\{C_{\{i,j\}} \rightarrow c_{\{i,j\}}\}$  that define a point in the border basis scheme, and produces the corresponding border basis.

```
makeBorBasisCorrespToCCoords[subList_, basisSet_, bdry_] :=
Module[{i, j, numBasis, numBdry, ijIndex},
(
numBasis = Length[basisSet];
numBdry = Length[bdry];
Table[bdry[[j]] -  $\sum_{i=1}^{\text{numBasis}} C_{\{i,j\}} \text{basisSet}[[i]], \{j, 1, \text{numBdry}\}] /. \text{subList}$ 
)];
```

---

### III. Functions for computing tangent space dimensions at

points  $[I]$  such that  $I$  has a border basis.

The next function constructs a list of all tangent space relations associated to a basis of linear syzygies (which generate the complete syzygy module) of the border basis of  $I$ . Recall that each syzygy gives rise to  $\mu$  relations, one for each monomial in the order ideal (or basis set). The function returns a tuple containing  $\{aLst, grandListOfTanSpaceRelns\}$ , where  $aLst$  is a list of indeterminates  $a_{\{i,j\}}$  that represent the tuple of the “generic tangent vector,” and  $grandListOfTanSpaceRelns$  is the desired list of tangent space relations, which are represented as tuples of scalars  $(c_{\{i,j\}})$  such that  $(\sum_{\{i,j\}} c_{\{i,j\}} \cdot a_{\{i,j\}}) = 0$  for all tangent vectors, which are encoded as tuples of scalars  $(a_{\{i,j\}})$ , as explained in Section 4 of the paper.

```

makeTanSpaceRelns[borBasis_, basisSet_, bdry_, varList_] :=
Module[{result, tanVecLst, numBasis, numBdry, aLst, numAs,
  nbrSyzygies, numSyz, i, j, k, z, curSyz, syzAppliedToTanVec,
  coeffs, curTanSpaceRelns, grandListOfTanSpaceRelns},
(
  numBasis = Length[basisSet];
  numBdry = Length[bdry];
  n = Length[varList];

  (* tanVecLst is the list of images (v(g1), v(g2), ..., v(gv))
  where v is a "generic tangent vector," gi are the border
  basis elements, and the images lie in basisSet. *)
  tanVecLst = Table[ $\sum_{i=1}^{\text{numBasis}}$  (a{i,j} basisSet[[i]]), {j, 1, numBdry}];
  aLst = Flatten[Table[a{i,j}, {j, 1, numBdry}, {i, 1, numBasis}]];
  numAs = Length[aLst];
  nbrSyzygies = makeLinearSyzygies[bdry, borBasis, varList];
  numSyz = Length[nbrSyzygies];

  grandListOfTanSpaceRelns = {};

  For[z = 1, z ≤ numSyz, z++,
    ( (* For each syzygy, find the associated tangent space relations,
    and add them to the growing list of these. We do this by
    applying the syzygy to tanVecLst, reducing modulo the borBasis,
    and finding the coefficients of the basis monomials in the
    resulting expression (which must be 0 modulo the border basis). *)
    curSyz = nbrSyzygies[[z]];
    syzAppliedToTanVec = reducePoly[curSyz.tanVecLst, bdry, borBasis, varList];
    coeffs = makeCoeffLst[syzAppliedToTanVec, basisSet, varList];
    curTanSpaceRelns =
      Table[Coefficient[coeffs[[j]], aLst[[k]], {j, 1, numBasis}, {k, 1, numAs}];
    grandListOfTanSpaceRelns = Join[grandListOfTanSpaceRelns, curTanSpaceRelns];
  );

  result = {aLst, grandListOfTanSpaceRelns}
)];

```

The next function finds the dimension of the tangent space at the point  $[I]$ . We assume that the user has separately executed the **makeTanSpaceRelns**

### function to obtain the aLst and list of tanSpRelns

```
tanSpaceDim[aLstLength_, tanSpRelns_] := Module[{result, rankOfRelns},
  (
    rankOfRelns = MatrixRank[tanSpRelns];
    result = aLstLength - rankOfRelns;
    result
  )];
```

## IV. Functions for working with distinguished ideals and related border (pre)bases. Distinguished ideals are defined in section 3 of the paper “Some elementary components of the Hilbert scheme of points.”

The following function constructs a lex-segment complement order ideal containing  $h_k$  monomials of degree  $k$ , for  $0 \leq k \leq s$ . The inputs are the Hilbert function  $H = \{1, h_1, \dots, h_s\}$  of the desired order ideal, and the list of variables. Recall that lists in *Mathematica* are indexed starting with 1 (one, not zero), so the degree of the monomials associated to the  $i$ th position in  $H$  is  $i - 1$ .

```
makeOrderIdeal[H_, varList_] := Module[{numH, numVars, result, i, numToTake},
  (
    numH = Length[H];
    numVars = Length[varList];
    result = {};
    For[i = 1, i ≤ numH, i++,
      (
        numToTake = H[[i]];
        result = Join[result, Take[allDegNMonoms[i - 1, numVars, 1], -numToTake]];
      )];
    result
  )];
```

Examples:

```

varList = Table[xi, {i, 1, 4}]
{ $x_1, x_2, x_3, x_4$ }

OO = makeOrderIdeal[{1, 4, 3, 2}, varList]
{1,  $x_1, x_2, x_3, x_4, x_3^2, x_3 x_4, x_4^2, x_3 x_4^2, x_4^3$ }

```

The following functions accept an order ideal (or basis set) and its boundary as input, and return the list of maximal basis monomials (resp. minimal boundary monomials) of that basis set. (The terms are defined in section 2.5 of the paper.)

A basis monomial is **maximal** if multiplication by EVERY variable takes it outside the basis set.

```

maxBasisMons[basisSet_, bdry_, varList_] :=
Module[{result, i, j, okSoFar, numVars, numBasis, curBasisMon},
(
result = {};
numBasis = Length[basisSet];
numVars = Length[varList];
For[i = 1, i ≤ numBasis, i++,
(
curBasisMon = basisSet[[i]];
okSoFar = True;
j = 1;
While[okSoFar && j ≤ numVars,
(
okSoFar = MemberQ[bdry, varList[[j]] * curBasisMon];
j = j + 1;
)];
If[okSoFar,
(
result = Append[result, curBasisMon];
)];
)];
result = sortInLexOrder[result, varList];
result
)];

```

OO

```

{1,  $x_1, x_2, x_3, x_4, x_3^2, x_3 x_4, x_4^2, x_3 x_4^2, x_4^3$ }

```

```

bdry = bdryMonoms[OO, varList]
{ $x_1^2$ ,  $x_1 x_2$ ,  $x_1 x_3$ ,  $x_1 x_4$ ,  $x_2^2$ ,  $x_2 x_3$ ,  $x_2 x_4$ ,  $x_1 x_3^2$ ,  $x_1 x_3 x_4$ ,  $x_1 x_4^2$ ,  $x_2 x_3^2$ ,
 $x_2 x_3 x_4$ ,  $x_2 x_4^2$ ,  $x_3^3$ ,  $x_3^2 x_4$ ,  $x_1 x_3 x_4^2$ ,  $x_1 x_4^3$ ,  $x_2 x_3 x_4^2$ ,  $x_2 x_4^3$ ,  $x_3^2 x_4^2$ ,  $x_3 x_4^3$ ,  $x_4^4$ }

maxes = maxBasisMons[OO, bdry, varList]
{ $x_1$ ,  $x_2$ ,  $x_3^2$ ,  $x_3 x_4^2$ ,  $x_4^3$ }

```

A boundary monomial is **minimal** if division by every variable that divides the monomial yields a basis monomial.

```

minBdryMons[basisSet_, bdry_, varList_] :=
Module[{result, i, j, okSoFar, numBdry, numVars, curBdryMon},
(
result = {};
numBdry = Length[bdry];
numVars = Length[varList];
For[i = 1, i ≤ numBdry, i++,
(
curBdryMon = bdry[[i]];
okSoFar = True;
j = 1;
While[okSoFar && j ≤ numVars,
(
If[Exponent[curBdryMon, varList[[j]]] > 0,
(
okSoFar = (MemberQ[basisSet, curBdryMon / varList[[j]]]);
)]];
j = j + 1;
)];
If[okSoFar,
(
result = Append[result, curBdryMon];
)];
result = sortInLexOrder[result, varList];
result
)];

```

Example:

OO

```

{1,  $x_1$ ,  $x_2$ ,  $x_3$ ,  $x_4$ ,  $x_3^2$ ,  $x_3 x_4$ ,  $x_4^2$ ,  $x_3 x_4^2$ ,  $x_4^3$ }

```

**bdry**

$$\{x_1^2, x_1 x_2, x_1 x_3, x_1 x_4, x_2^2, x_2 x_3, x_2 x_4, x_1 x_3^2, x_1 x_3 x_4, x_1 x_4^2, x_2 x_3^2, x_2 x_3 x_4, x_2 x_4^2, x_3^3, x_3^2 x_4, x_1 x_3 x_4^2, x_1 x_4^3, x_2 x_3 x_4^2, x_2 x_4^3, x_3^2 x_4^2, x_3 x_4^3, x_4^4\}$$

**mins = minBdryMons[OO, bdry, varList]**

$$\{x_1^2, x_1 x_2, x_1 x_3, x_1 x_4, x_2^2, x_2 x_3, x_2 x_4, x_3^3, x_3^2 x_4, x_3 x_4^3, x_4^4\}$$

The next function (which has two versions) constructs the “short list” of generators of a distinguished ideal using the leading and trailing monomial sets LM and TM as described in section 3 of the paper. The first version generates coefficients +1, −1, or 0 with equal probability; the second, which requires an additional parameter  $p$ , generates a random nonzero coefficient of −1 with probability  $p$ , and 0 with probability  $1 - p$ .

```
makeShortListOfIdealGenerators[LM_, TM_] := Module[{result, i, j, numLM, numTM},
  (
    numLM = Length[LM];
    numTM = Length[TM];

    result = Table[LM[[i]] -  $\left(\sum_{j=1}^{\text{numTM}} \text{RandomInteger}[\{-1, 1\}] \text{TM}[[j]]\right)$ , {i, 1, numLM}]
  )];
```

```

makeShortListOfIdealGenerators[LM_, TM_, p_] :=
Module[{result, i, j, numLM, numTM, coeffLst},
(
numLM = Length[LM];
numTM = Length[TM];
result = {};
For[i = 1, i ≤ numLM, i++, (
coeffLst = Table[If[RandomReal[] < p, 1, 0], {j, 1, numTM}];
result = Append[result, LM[[i]] -  $\left(\sum_{j=1}^{\text{numTM}} \text{coeffLst}[[j]] * \text{TM}[[j]]\right)$ ];
);
result
)]];

```

Examples:

**maxes**

$\{x_1, x_2, x_3^2, x_3 x_4^2, x_4^3\}$

**mins**

$\{x_1^2, x_1 x_2, x_1 x_3, x_1 x_4, x_2^2, x_2 x_3, x_2 x_4, x_3^3, x_3^2 x_4, x_3 x_4^3, x_4^4\}$

**LM = Take[mins, 7]**

$\{x_1^2, x_1 x_2, x_1 x_3, x_1 x_4, x_2^2, x_2 x_3, x_2 x_4\}$

**TM = Take[maxes, -3]**

$\{x_3^2, x_3 x_4^2, x_4^3\}$

**makeShortListOfIdealGenerators[LM, TM, .67]**

$\{x_1^2 - x_3^2 - x_3 x_4^2, x_1 x_2 - x_3^2 - x_3 x_4^2 - x_4^3, x_1 x_3 - x_3^2 - x_3 x_4^2 - x_4^3,$   
 $-x_3^2 + x_1 x_4 - x_3 x_4^2, x_2^2 - x_3^2 - x_4^3, x_2 x_3 - x_3^2 - x_4^3, -x_3^2 + x_2 x_4 - x_3 x_4^2\}$

**G = makeShortListOfIdealGenerators[LM, TM]**

$\{x_1^2 + x_4^3, x_1 x_2 - x_3^2 + x_3 x_4^2 + x_4^3, x_1 x_3 - x_3^2 + x_4^3,$   
 $x_1 x_4 + x_4^3, x_2^2 - x_3^2 - x_4^3, x_2 x_3 + x_3^2 + x_3 x_4^2, x_2 x_4 - x_3 x_4^2 + x_4^3\}$

The following function constructs an O-border basis by adding to the short list of generators *G* the boundary monomials that do not lie in the set of leading



monomials “LM.” The terminology is discussed in section 3 of the paper. In the resulting border (pre)basis, the elements of  $G$  have the same list positions (or indices) as their corresponding leading monomials have in the list of boundary monomials.

It is useful and important for the border basis to be in the same order as the corresponding monomials in  $\text{bdry}$ . So, the function for building the border basis (or at least border pre-basis) needs to achieve this. This function accepts the short list of generators of a distinguished ideal -- one constructed using LM and TM as in section 3 of the paper -- we know that for such ideals, if we add to the short list all of the boundary monomials that are not in LM, then we get a border basis. IF the short list generates the same ideal as the full border basis does, then the ideal is said to be **efficient**.

```
makeBorderBasisOfI[G_, bdry_, LM_] :=
Module[{i, j, result, numBdry, curBdryMon, loc},
(
result = {};
numBdry = Length[bdry];
For[i = 1, i <= numBdry, i++,
(
curBdryMon = bdry[[i]];
If[MemberQ[LM, curBdryMon],
(
loc = Position[LM, curBdryMon][[1]][[1]];
result = Append[result, G[[loc]]];
),
(
result = Append[result, curBdryMon];
)]];
result
)];
```

OO

$$\{1, x_1, x_2, x_3, x_4, x_3^2, x_3 x_4, x_4^2, x_3 x_4^2, x_4^3\}$$

TM

$$\{x_3^2, x_3 x_4^2, x_4^3\}$$

LM

$$\{x_1^2, x_1 x_2, x_1 x_3, x_1 x_4, x_2^2, x_2 x_3, x_2 x_4\}$$

**G**

$$\{x_1^2 + x_4^3, x_1 x_2 - x_3^2 + x_3 x_4^2 + x_4^3, x_1 x_3 - x_3^2 + x_4^3, \\ x_1 x_4 + x_4^3, x_2^2 - x_3^2 - x_4^3, x_2 x_3 + x_3^2 + x_3 x_4^2, x_2 x_4 - x_3 x_4^2 + x_4^3\}$$

**bdry**

$$\{x_1^2, x_1 x_2, x_1 x_3, x_1 x_4, x_2^2, x_2 x_3, x_2 x_4, x_1 x_3^2, x_1 x_3 x_4, x_1 x_4^2, x_2 x_3^2, \\ x_2 x_3 x_4, x_2 x_4^2, x_3^3, x_3^2 x_4, x_1 x_3 x_4^2, x_1 x_4^3, x_2 x_3 x_4^2, x_2 x_4^3, x_3^2 x_4^2, x_3 x_4^3, x_4^4\}$$

**borBasis = makeBorderBasisOfI[G, bdry, LM]**

$$\{x_1^2 + x_4^3, x_1 x_2 - x_3^2 + x_3 x_4^2 + x_4^3, x_1 x_3 - x_3^2 + x_4^3, x_1 x_4 + x_4^3, \\ x_2^2 - x_3^2 - x_4^3, x_2 x_3 + x_3^2 + x_3 x_4^2, x_2 x_4 - x_3 x_4^2 + x_4^3, x_1 x_3^2, x_1 x_3 x_4, x_1 x_4^2, x_2 x_3^2, \\ x_2 x_3 x_4, x_2 x_4^2, x_3^3, x_3^2 x_4, x_1 x_3 x_4^2, x_1 x_4^3, x_2 x_3 x_4^2, x_2 x_4^3, x_3^2 x_4^2, x_3 x_4^3, x_4^4\}$$

The following function accepts the short list of generators  $G$ , the set of leading monomials  $LM$ , and the list of boundary monomials  $bdry$ , and returns TRUE if the distinguished ideal  $I$  associated to  $G$  is efficient (that is,  $I = (G)$ ), and FALSE otherwise. It tests the condition given in the paper (in section 3.2):  $I = (G)$  is efficient if and only if every boundary monomial not in  $LM$  lies in  $I$ .

```
isEfficient[G_, LM_, bdry_, varList_] :=
Module[{result, okSoFar, gb, bdryMonsToCheck, numToCheck, remainder, i},
(
gb = GroebnerBasis[G, varList];
bdryMonsToCheck = Complement[bdry, LM];
numToCheck = Length[bdryMonsToCheck];

remainder = 0;
okSoFar = (SameQ[remainder, 0]);
i = 1;
While[(okSoFar) && (i ≤ numToCheck),
(
remainder = PolynomialReduce[bdryMonsToCheck[[i]], gb, varList][[2]];
okSoFar = (SameQ[remainder, 0]);
i = i + 1;
)];
result = okSoFar;
result
)];
```

```
isEfficient[G, LM, bdry, varList]
True
```

We use the following function to construct the sets “partial L” and “partial T” (this is used in the function **isThetaEfficient**).

```
partialMonomSet[monSet_, varList_] := Module[{result, numVars},
  (
    numVars = Length[varList];
    result = sortInLexOrder[DeleteDuplicates[
      Flatten[Table[varList[[i]] * monSet, {i, 1, numVars}]]], varList]
  )];
partialMonomSet[{1, x1, x2}, {x1, x2, x3}]
{x1, x2, x3, x12, x1 x2, x1 x3, x22, x2 x3}
```

The next function tests a given distinguished ideal with short list  $G$  for theta-efficiency (defined in section 3.2). If the parameter “verbose” is False, only the True/False output is displayed; if “verbose” is True, additional information is displayed that will assist the user in determining why the given ideal fails to be theta-efficient, if it does.

```
isThetaEfficient[G_, LM_, TM_, bdry_, varList_, verbose_] :=
Module[{result, bdryLM, bdryTM, i, j, nonLeadingBdryMons,
  Q, numQ, prods, numProds, numVars, okSoFar, monomsToTest,
  isEmpty, curQMonom, isMultiple, monsToRemove, thetaMatrix},
  (
    numVars = Length[varList];
    Q = DeleteDuplicates[
      Join[partialMonomSet[LM, varList], partialMonomSet[TM, varList]]];
    numQ = Length[Q];
    nonLeadingBdryMons = Complement[bdry, LM];
    okSoFar = True;
    (* First we check that each non-
      leading bdry monomial is divisible by one of the Q *)
    (* If that is false, we can quit. If it is true,
      then we go on to see that the number of products is larger
      than the number of targets, and that the linear map sigma is onto. If
      both of the latter conditions hold, the ideal is theta-efficient. *)
```

```
(* The following loop removes from the set of non-leading boundary monomials
   all that are multiples of monomials in Q.  If the result is the empty set,
   then condition (1) of Lemma 3.1 holds, so okSoFar should still be true. *)
```

```
i = 1;
monomsToTest = nonLeadingBdryMons;
isEmpty = (Length[monomsToTest] == 0);
isMultiple[mon_] := monomDivides[curQMonom, mon, varList];
```

```
While[(!isEmpty) && (i ≤ numQ),
  (
    curQMonom = Q[[i]];
    monsToRemove = Select[monomsToTest, isMultiple];
    monomsToTest = Complement[monomsToTest, monsToRemove];
    isEmpty = (Length[monomsToTest] == 0);
    i = i + 1;
  )];
okSoFar = isEmpty;
```

```
If[verbose,
  (
    If[okSoFar,
      (
        Print["Condition 1 of Proposition 3.1 is True."];
      ),
      (
        Print["Condition 1 of Proposition 3.1 is False."];
      )
    ]];
)];
```

```
(* If we are still OK,
   we proceed to check if the map theta is surjective or not. *)
```

```
If[okSoFar,
  (
    prods = Flatten[Table[varList[[i]] * G, {i, 1, numVars}]];
    numProds = Length[prods];
    okSoFar = numProds ≥ numQ;

    If[verbose,
      (
        If[okSoFar,
          (
            Print["(numProds = ", numProds, ") ≥ (numQ = ", numQ, ")"];
          )
        ]
      )
    ]
  )
];
```

```

    ),
    (
        Print["(numProds = ", numProds, ") < (numQ = ", numQ, ")"];
    )];
];

If[okSoFar,
    (
        (* Construct the matrix of the map and
           check for surjectivity -- i.e. matrix has maximal rank *)
        thetaMatrix = Transpose[makeListOfCoeffLsts[prods, Q, varList]];
        okSoFar = MatrixRank[thetaMatrix] == numQ;
    )];

If[verbose,
    (
        If[okSoFar,
            (
                Print["The map  $\phi$  is surjective."];
            ),
            (
                Print["The map  $\phi$  is not surjective."];
            )];
    )];

];

result = okSoFar

];

```

## V. Functions used in implementing the test for plausible genericity of shapes $(n, K, r, s)$ .

In this section of the notebook we write code to implement the test (discussed in section 10 of the paper) for a sufficiently general distinguished ideal of shape  $(n, \kappa, r, s)$  to be plausibly generic. Through-

out this section, the inputs to a function always include the four components of the shape:  $\{n, \kappa, r, s\}$ , and occasionally another input such as a particular degree. See sections 9 and 10 of the paper for further discussion.

## The order ideal and its boundary

Given the four inputs, the following function constructs the associated order ideal.

```
ordIdeal[n_, κ_, r_, s_] := Module[{result, i, j},
  (
    result = {};
    For[i = 0, i < r, i++,
      (
        result = Join[result, allDegNMonoms[i, n, 1]];
      )
    ];

    For[i = r, i ≤ s, i++,
      (
        result = Join[result, allDegNMonoms[i, n, n - κ + 1]];
      )
    ];

    result
  )];
```

```
OO = ordIdeal[4, 2, 2, 3]
```

```
{1, x1, x2, x3, x4, x32, x3 x4, x42, x33, x32 x4, x3 x42, x43}
```

```
varList = {x1, x2, x3, x4};
```

The boundary can then be constructed using the utility function **bdryMonoms**.

```
varList
```

```
{x1, x2, x3, x4}
```

```
bdry = bdryMonoms[OO, varList]
```

```
{x12, x1 x2, x1 x3, x1 x4, x22, x2 x3, x2 x4, x1 x32, x1 x3 x4, x1 x42, x2 x32, x2 x3 x4, x2 x42, x1 x33,
  x1 x32 x4, x1 x3 x42, x1 x43, x2 x33, x2 x32 x4, x2 x3 x42, x2 x43, x34, x33 x4, x32 x42, x3 x43, x44}
```

Next we have functions for computing the number of leading (boundary) and the number of trailing (basis) monomials:

```
numLeading[n_, κ_, r_, s_] := Binomial[n - 1 + r, r] - Binomial[κ - 1 + r, r]
λ = numLeading[4, 2, 2, 3]
7

numTrailing[n_, κ_, r_, s_] := Binomial[κ - 1 + s, s]
τ = numTrailing[4, 2, 2, 3]
4
```

## Functions for the number of basis and boundary monomials of each degree, and overall

This function computes the number of basis monomials of degree  $0 \leq d \leq s$ :

```
numBasisMonsOfDeg[d_, n_, κ_, r_, s_] :=
  If[d ≤ r - 1, Binomial[n - 1 + d, d], Binomial[κ - 1 + d, d]]
Hence the total number of basis monomials is given by
numBasisMons[n_, κ_, r_, s_] :=  $\sum_{d=0}^s$  numBasisMonsOfDeg[d, n, κ, r, s]
```

The next function computes the number of boundary monomials of degree  $r \leq d \leq s + 1$ . (The boundary monomials are listed and counted in Section 9.2 of the paper.)

```
numBdryMonsOfDeg[d_, n_, κ_, r_, s_] :=
  Which[d == r,
    (
      Binomial[n - 1 + r, r] - Binomial[κ - 1 + r, r]
    ),
    (d > r) && (d < s + 1),
    (
      (n - κ) * Binomial[κ - 1 + d - 1, d - 1]
    ),
    (d == s + 1),
    (
      (n - κ) * Binomial[κ - 1 + s, s] + Binomial[κ - 1 + s + 1, s + 1]
    )
  ];
```

Hence the total number of boundary monomials is given by

```
numBdryMons[n_, κ_, r_, s_] := Sum[numBdryMonsOfDeg[d, n, κ, r, s], {d, r, s+1}]
```

```
numBasisMons[5, 2, 2, 3]
```

```
13
```

```
numBdryMons[5, 2, 2, 3]
```

```
38
```

## Functions for computing the number of independent linear syzygies $\psi$ .

Section 2.3 describes how to do this; the answer is  $v \cdot (n+1) - |T|$ , where  $T$  is the set of target monomials. The next function counts the target monomials for distinguished ideals of shape  $(n, \kappa, r, s)$ , as discussed in Section 9.3 of the paper.

```
numTargets[n_, κ_, r_, s_] := Module[{ },
  (
    Binomial[n-1+r, r] - Binomial[κ-1+r, r] +

    Binomial[n+r, r+1] - Binomial[κ+r, r+1] +

    Sum[
      ((n-κ) * (Binomial[κ-1+d-1, d-1]) +
      (Binomial[n-κ-1+2, 2]) * (Binomial[κ-1+d-2, d-2])) +

      Binomial[κ-1+s+1, s+1] + (n-κ) * Binomial[κ-1+s, s] +
      Binomial[n-κ-1+2, 2] * Binomial[κ-1+s-1, s-1] +

      Binomial[κ-1+s+2, s+2] + (n-κ) * Binomial[κ-1+s+1, s+1] +
      Binomial[n-κ-1+2, 2] * Binomial[κ-1+s, s]
    ], {d, r+2, s}
  );
```

Therefore the number of independent neighbor syzygies is given by

```
numNeighborSyzygies[n_, κ_, r_, s_] :=
  (n+1) numBdryMons[n, κ, r, s] - numTargets[n, κ, r, s];
```

```
numNeighborSyzygies[5, 2, 2, 3]
```

```
105
```



## Number of tangent space relations

The following function computes the number of tangent space relations in a given degree  $0 \leq d \leq s$ :

```
numTanSpaceRelnsInDeg[d_, n_, κ_, r_, s_] :=  
  numNeighborSyzygies[n, κ, r, s] * numBasisMonsOfDeg[d, n, κ, r, s];
```

Therefore, the total number of tangent space relations is given by

$$\text{numTanSpaceRelns}[n_, \kappa_, r_, s_] := \sum_{d=0}^s \text{numTanSpaceRelnsInDeg}[d, n, \kappa, r, s]$$

## Upper bound on the rank of the tangent space relations in degree $d$

As Section 9.5 explains, the tangent space relations of degree  $d$  have a rank that is bounded above by the number of  $a_{\{i,j\}}$  that can appear in those relations (the set of such  $a_{\{i,j\}}$  is called  $A_d$  in the paper).

The following function returns  $|A_d|$ ; the formulas are given in Lemma 9.5:

```

numAsInTanSpReInnsOfDeg[d_, n_,  $\kappa$ _, r_, s_] := Module[{v,  $\lambda$ , result},
  (
    v = numBdryMons[n,  $\kappa$ , r, s];
     $\lambda$  = numLeading[n,  $\kappa$ , r, s];

    result = Which[
      0 ≤ d ≤ r - 1,
      (
        (v -  $\lambda$ ) * Binomial[n - 1 + d, d] + v * Binomial[n - 1 + d - 1, d - 1]
      ),
      d == r,
      (
        (v -  $\lambda$ ) * Binomial[ $\kappa$  - 1 + r, r] + v * Binomial[ $\kappa$  - 1 + r - 1, r - 1]
      ),
      r + 1 ≤ d ≤ s - 1,
      (
        (v -  $\lambda$ ) * Binomial[ $\kappa$  - 1 + d, d] + v * Binomial[ $\kappa$  - 1 + d - 1, d - 1]
      ),
      d == s,
      (
        (v -  $\lambda$ ) * Binomial[ $\kappa$  - 1 + s, s] +
        v * Binomial[ $\kappa$  - 1 + s - 1, s - 1] + v * Binomial[n - 1 + r - 1, r - 1]
      )
    ];

    result
  )];

```

---

## Test to see if there are enough tangent space relations for full rank in each degree

The next function returns **True** if there are enough tangent space relations to achieve the maximum possible rank in each degree  $0 \leq d \leq s$ , and **False** otherwise.

```

hasEnoughReIns[n_, κ_, r_, s_] := Module[{result, okSoFar, d},
  (
    okSoFar = True;
    d = 0;
    While[(d ≤ s) && (okSoFar),
      (
        okSoFar =
          numTanSpaceReInsInDeg[d, n, κ, r, s] ≥ numAsInTanSpReInsOfDeg[d, n, κ, r, s];
        If[okSoFar,
          (
            d = d + 1;
          )];
      )];
    result = okSoFar;
    result
  )];

hasEnoughReIns[6, 3, 2, 3]

True

```

---

## Test for $\vartheta$ -efficiency

The following function returns **True** if sufficiently general distinguished ideals of the given shape are likely to be  $\vartheta$ -efficient, and **False** otherwise. That is, **True** is returned if and only if the domain of the map  $\vartheta$  has dimension  $(n \cdot \lambda)$  greater than or equal to the dimension of the codomain  $(= |Q| = |\partial LE \cup \partial TR|)$ . (Recall that we are assuming that  $r < s$ ).

```

thetaEfficiencyIsLikely[n_, κ_, r_, s_] :=
  n (numLeading[n, κ, r, s]) ≥ Binomial[n - 1 + r + 1, r + 1] - Binomial[κ - 1 + r + 1, r + 1] +
    (n - κ) Binomial[κ - 1 + s, s] + Binomial[κ - 1 + s + 1, s + 1];

```

---

## Test for plausible genericity

The following function returns **True** if sufficiently general distinguished ideals of the given shape are likely to be generic, meaning that they have enough tangent space relations in all degrees to achieve the maximum possible rank in each degree and are  $\sigma'$ -efficient. (We test for  $\sigma'$ -efficiency since it is much more computationally efficient to do so than to test for efficiency).

```

genericityIsPlausible[n_, κ_, r_, s_] :=
  thetaEfficiencyIsLikely[n, κ, r, s] && hasEnoughReIns[n, κ, r, s];

```

```
genericityIsPlausible[5, 2, 2, 3]
```

```
True
```

```
genericityIsPlausible[6, 3, 2, 3]
```

```
False
```
